# Supplementary material for: Floquet-engineered dissipative stabilizer pumping in neutral atom arrays
Source: arXiv:2509.18379 source file (2026-11-26)
Supplement: Supplementary file 1 [file SM.tex]

%% ****** Start of file apsguide4-1.tex ****** %
%%
%%   This file is part of the APS files in the REVTeX 4.1 distribution.
%%   Version 4.1r of REVTeX, August 2010.
%%
%%   Copyright (c) 2009, 2010 The American Physical Society.
%with the   See the REVTeX 4.1 README file for restrictions and more information.
%%
\documentclass[pra,aps,amsmath,amssymb,amsfonts,nofootinbib,longbibliography,superscriptaddress]{revtex4-2}%,
\usepackage{graphicx,subfigure,amsmath}%
\usepackage{color}
\usepackage[bookmarks=false]{hyperref}
\hypersetup{colorlinks=true,citecolor=blue,linkcolor=blue,urlcolor=blue,pdfstartview=FitH,bookmarksopen=true}
\setlength{\textheight}{9.5in}
\usepackage{amsmath,amstext}
\usepackage{graphicx}
\usepackage{booktabs}
\usepackage{multirow}
\usepackage{braket}
\definecolor{green}{rgb}{0.8,0.98,0.83}
%\pagecolor{green}
\usepackage{float}
\usepackage{mathrsfs}
\usepackage{graphicx}
\usepackage{xcolor}
\newcommand{\gmp}{\gamma_{p}}
\newcommand{\omp}{\Omega_{p}}
\newcommand{\kpp}{\kappa}
\setcounter{equation}{0}
% —— 编号加 S —— 

% 章节用罗马数字

\usepackage{braket} % For Dirac notation \ket{} and \bra{}
% Define a new operator for the real part

\makeatletter
  % 文末列表标签 [S1]
  % 正文引用数字 S1 -> [S1]
\makeatother

\begin{document}

\title{ Supplemental Material:
Scalable Steady-State Entanglement with Floquet-Engineered Stabilizer Pumping in Neutral Atom Arrays}

\author{F. Q. Guo}
\affiliation{Center for Quantum Science and School of Physics, Northeast Normal University, Changchun 130024, China}

\author{Shi-Lei Su}
\email{slsu@zzu.edu.cn}
\affiliation{School of Physics, Key Laboratory of Materials Physics of Ministry of Education, and International Laboratory for Quantum Functional Materials of Henan, Zhengzhou University, Zhengzhou 450001, China}
\affiliation{Institute of Quantum Materials and Physics, Henan Academy of Science, Henan 450046, China}

\author{Weibin Li}
\email{weibin.li@nottingham.ac.uk}
\affiliation{School of Physics and Astronomy, and Centre for the Mathematics and Theoretical Physics of Quantum nonequilibrium Systems, The University of Nottingham, Nottingham NG7 2RD, United Kingdom}

\author{X. Q. Shao}
\email{shaoxq644@nenu.edu.cn}
\affiliation{Center for Quantum Science and School of Physics, Northeast Normal University, Changchun 130024, China}
\affiliation{Institute of Quantum Science and Technology, Yanbian University, Yanji 133002, China}

\maketitle

\section{Derivation of Effective Hamiltonian}\label{sec:eff_Ham}

\subsection{Effective Hamiltonian via Zeno Dynamics}

To obtain a pumping resistant to Doppler dephasing and position fluctuation errors, we provide a control sequence using unitary kicks~\cite{Facchi2004Unification, Facchi2008Quantum}. 
The system alternates two driving Hamiltonians over \(\mathcal{N}\) cycles, described by
\begin{eqnarray}\label{eq_fullspace}
H_{\text{total}}(t) =
\begin{cases}
H_{a} \equiv \sum_i \frac{\Omega_a}{2} |r_i\rangle\langle G_i| + \text{H.c.} + H_V, & t \in [nT, nT + t_a), \\
H_{b}(t) \equiv\sum_i \frac{\Omega_b}{2} e^{i \Delta t} |r_i\rangle\langle G_i| + \text{H.c.} + H_V, & t \in [nT + t_a, nT+T),
\end{cases}
\end{eqnarray}
where \(n = 0, 1, \dots, \mathcal{N}-1\) is the cycle index and \(H_V = \sum_{i<j} U_{rr} |r_i\rangle\langle r_i| \otimes |r_j\rangle\langle r_j|\) represents the Rydberg interaction between atoms with $U_{rr}=-C_{6}/R^6$. Each cycle of duration \(T = t_a + t_b\) consists of the system Hamiltonian \(H_{a}\) acting for time \(t_a\) with evolution \(U_{a}(t_a) = \exp(-i H_{a} t_{a})\), followed by the kick Hamiltonian \(H_{b}\) acting for time \(t_b\) with evolution \(U_{b}(t_b) = \mathcal{T}\exp[-i \int_0^{t_b} H_{b}(t) \, dt]\). The total system evolution is given by \(U_{\mathcal{N}}(T) = [U_{b}(t_b) U_{a}(t_a)]^{\mathcal{N}}\). In particular, we can find $i (d/dt_a)\mathcal{V}_{\mathcal{N}}(t_a)=H_{\mathcal{N}}(t_a)\mathcal{V}_{\mathcal{N}}(t_a)$ with $\mathcal{V}_{\mathcal{N}}(t_a) = U_{b}^{\dagger \mathcal{N}}(t_b)U_{\mathcal{N}}(T)$, $\mathcal{V}_{\mathcal{N}}(0) = \mathcal{I}$ being identity, and $H_{\mathcal{N}}(t_a) = 1/\mathcal{N}\sum_{n=0}^{\mathcal{N}-1}U_{b}^{\dagger \mathcal{N}}(U_{b}U_{a})^{n}U_{b}H_{a}U_{a}^{\dagger}(U_{b}U_{a})^{\dagger n}U_{b}^{\mathcal{N}}$. Considering the conditions $\Omega_{b}t_{b}\gg \Omega_{a}t_{a}$ and large-$\mathcal{N}$ limit, we can obtain the limiting evolution operator~\cite{Shao2011Quantum}
\begin{equation}
    \mathcal{U}(t_a)\equiv \lim_{\mathcal{N}\to\infty}\mathcal{V}_{\mathcal{N}}(t_a),
\end{equation}
satisfying the equation $i\frac{d}{dt}\mathcal{U}(t)=H_{Z}\mathcal{U}(t)$, with $\mathcal{U}(0) = \mathcal{I}$ and ``Zeno" Hamiltonian $H_{Z}\equiv \lim_{\mathcal{N}\to \infty} H_{\mathcal{N}}(t) \sim \lim_{\mathcal{N}\to \infty}\frac{1}{\mathcal{N}}\sum_{n=0}^{\mathcal{N}-1}U_{b}^{\dagger n}H_{a}U_{b}^{n}$. Assuming $U_{b}(t_b) = \sum_{\mu}\lambda_{\mu}(t_b)P_{\mu}(t_b)$ with $\lambda_{\mu}(t_b)$ and $P_{\mu}(t_b)$ eigenvalue and eigenprojector related to time $t_b$. Consequently,
\begin{eqnarray}\label{eq:Zeno_Hamiltonain}
    H_{Z} &=& \sum_{\mu}P_{\mu}H_{a}P_{\mu}.
\end{eqnarray}

As a result, the evolution operation can be presented as 
\begin{eqnarray}\label{eq_UN}
    U_{\mathcal{N}}(T) &\sim& U_{b}^{\mathcal{N}}(t_b)\mathcal{U}^{\mathcal{N}}(t_a) = U_{b}^{\mathcal{N}}(t_b) \exp(-iH_{Z}\mathcal{N} t_a) = \exp[-i\sum_{\mu}\mathcal{N}(\lambda_{\mu}P_{\mu} + P_{\mu}H_{a}P_{\mu} t_a)].
\end{eqnarray}

Since \(H_b(t)\) is time-dependent, the Zeno Hamiltonian can be obtained numerically at any given moment from Eq.~(\ref{eq:Zeno_Hamiltonain}), but its analytical expression is generally intractable. To simplify the model, we impose the large-detuning condition and neglect the accompanying Stark shifts. This approximation effectively disregards the special cases where the eigenspectrum of $U_b(t_b)$ exhibits degeneracies near the eigenvalue $+1$, while still capturing the essential physics under typical conditions; quantitative deviations are evaluated through comparison with full numerical simulations.

The total Hamiltonian in the single-atom ground state subspace $\{|G\rangle, |r\rangle\}$ can be rewritten as
\begin{eqnarray}
    H_{a_{1}} &=& \frac{\Omega_{a}}{2}|r\rangle\langle G| + {\rm H.c.}, \cr\cr
    H_{b_{1}} &=& \frac{\Omega_{b}}{2} e^{i \Delta t} |r\rangle\langle G| + {\rm H.c.}
\end{eqnarray}
Under the circumstance of $\Delta \gg \{\Omega_a, \Omega_b\}$, $H_{b_1}\approx0$, the projectors from evolution operation $U_{b_1}$ are $P_{G}^{1} = |G\rangle \langle G|$ and $P_{r}^{1} = |r\rangle \langle r|$. The corresponding Zeno Hamiltonian is calculated as
\begin{eqnarray}
    H_{Z_1} &=& \frac{\Omega_\text{eff}}{2}|r\rangle\langle G| + {\rm H.c.},
\end{eqnarray}
with $\Omega_\text{eff} = \Omega_{a}t_a/(t_a + t_b)$ effective Rabi frequency.

Considering $U_{rr} = -\Delta$, the total Hamiltonian in the two-atom ground state subspace $\{|GG\rangle, |w\rangle, |rr\rangle\}$ with $|w\rangle = (|G r\rangle + |r G \rangle)/\sqrt{2}$ can be rewritten as
\begin{eqnarray}
    H_{a_{2}} &=& \frac{\Omega_{a}}{\sqrt{2}}(|w\rangle\langle GG| + |rr\rangle\langle w|) + {\rm H.c.} - \Delta |rr\rangle\langle rr|, \cr\cr
    H_{b_{2}} &=& \frac{\Omega_{b}}{\sqrt{2}} e^{i \Delta t} (|w\rangle\langle GG| + |rr\rangle\langle w|) + {\rm H.c.} - \Delta |rr\rangle\langle rr|,
\end{eqnarray}
Under the circumstance of $\Delta \gg \{\Omega_a, \Omega_b\}$, $H_{b_2}\approx{\Omega_{b}}/{\sqrt{2}}(|w\rangle\langle rr|+|rr\rangle\langle w|)$, the projectors from the evolution operation $U_{b_2}$ are $P^2_{0} = |GG\rangle \langle GG|$ and $P^2_{+} = \frac{1}{2}(|w\rangle\langle w| + |w\rangle\langle rr| + |rr\rangle\langle w| + |rr\rangle\langle rr|)$ and $P^2_- = \frac{1}{2}(|w\rangle\langle w| - |w\rangle\langle rr| - |rr\rangle\langle w| + |rr\rangle\langle rr|)$. The corresponding Zeno Hamiltonian $H_{Z_2}$ is calculated as 0.

The total Hamiltonian in the three-atom ground state subspace $\{|GGG\rangle, |w_{1}\rangle, |w_{2}\rangle, |rrr\rangle\}$ with $|w_{1}\rangle = (|GGr\rangle + |GrG\rangle + |rGG\rangle)/\sqrt{3}$, and $|w_{2}\rangle = (|Grr\rangle + |rGr\rangle + |rrG\rangle)/\sqrt{3}$ can be rewritten as
\begin{eqnarray}
    H_{a_{3}} &=& \frac{\Omega_{a}}{2}(\sqrt{3}|w_1\rangle\langle GGG| + 2|w_2\rangle\langle w_1| + \sqrt{3}|rrr\rangle\langle w_2|) + {\rm H.c.} - \Delta|w_2\rangle\langle w_2| - 3\Delta|rrr\rangle\langle rrr|,\cr\cr
    H_{b_{3}} &=& \frac{\Omega_{b}}{2}e^{i\Delta t}(\sqrt{3}|w_1\rangle\langle GGG| + 2| w_2\rangle\langle w_1| + \sqrt{3}|rrr\rangle\langle w_2|) + {\rm H.c.} - \Delta|w_2\rangle\langle w_2| - 3\Delta|rrr\rangle\langle rrr|.
\end{eqnarray}
Under the circumstance of $\Delta \gg \{\Omega_a, \Omega_b\}$, $H_{b_3}\approx{\Omega_{b}}(|w_1\rangle\langle w_2|+|w_2\rangle\langle w_1|)$, the projectors from evolution operation $U_{b_2}$ are $P^3_{0} = |GGG\rangle \langle GGG|$, $P_{rrr} = |rrr\rangle \langle rrr|$, $P^3_{+} = \frac{1}{2}(|w_{1}\rangle\langle w_{1}| + |w_{1}\rangle\langle w_{2}| + |w_{2}\rangle\langle w_{1}| + |w_{2}\rangle\langle w_{2}|)$, and $P^3_{-} = \frac{1}{2}(|w_{1}\rangle\langle w_{1}| - |w_{1}\rangle\langle w_{2}| - |w_{2}\rangle\langle w_{1}| + |w_{2}\rangle\langle w_{2}|)$. The corresponding Zeno Hamiltonian  $H_{Z_3}$ is calculated as 0.

\vspace{2em}  
\textbf{For pumping the two-qubit boundary stabilizer $S_{1}=X_{1}Z_{2}$, we require  }
\begin{eqnarray}
    H_{a}^{S_{1}} &=& \frac{\Omega_{a}}{2}(|r_{1}\rangle\langle -_{1}|\otimes\mathcal{I}_{2} + \mathcal{I}_{1}\otimes|r_{2}\rangle\langle 1_{2}|) + {\rm H.c.} + H_{V},\cr\cr
    H_{b}^{S_{1}}(t) &=& \frac{\Omega_{b}}{2}e^{i\Delta t}(|r_{1}\rangle\langle -_{1}|\otimes\mathcal{I}_{2} + \mathcal{I}_{1}\otimes|r_{2}\rangle\langle 1_{2}|) + {\rm H.c.} + H_{V}.\nonumber
\end{eqnarray}
The effective Zeno Hamiltonian can be obtained as
\begin{eqnarray}\label{eq:H_S1}
    H_{S_{1}} &=& \frac{\Omega_\text{eff}}{2}(|r_{1}0_{2}\rangle\langle -_{1}0_{2}| + |+_{1}r_{2}\rangle\langle +_{1}1_{2}|) + {\rm H.c.}
\end{eqnarray}

\vspace{2em}  
\textbf{For pumping the two-qubit boundary stabilizer $S_{N}=Z_{N-1}X_{N}$, we require }
\begin{eqnarray}
    H_{a}^{S_{N}} &=& \frac{\Omega_{a}}{2}(|r_{N-1}\rangle\langle 1_{N-1}|\otimes\mathcal{I}_{N} + \mathcal{I}_{N-1}\otimes|r_{N}\rangle\langle -_{N}|) + {\rm H.c.} + H_{V},\cr\cr
    H_{b}^{S_{N}}(t) &=& \frac{\Omega_{b}}{2}e^{i\Delta t}(|r_{N-1}\rangle\langle 1_{N-1}|\otimes\mathcal{I}_{N} + \mathcal{I}_{N-1}\otimes|r_{N}\rangle\langle -_{N}|) + {\rm H.c.} + H_{V}.\nonumber
\end{eqnarray}
The effective Zeno Hamiltonian can be obtained as
\begin{eqnarray}\label{eq:H_SN}
    H_{S_{N}} &=& \frac{\Omega_\text{eff}}{2}(|r_{N-1}+_{N}\rangle\langle 1_{N-1}+_{N}| + |0_{N-1}r_{N}\rangle\langle 0_{N-1}-_{N}|) + {\rm H.c.}
\end{eqnarray}

\vspace{2em}  
\textbf{Similarly, for pumping the three-qubit bulk stabilizer $S_{k}=Z_{k-1}X_{k}Z_{k+1}~(k=2,3,...,N-1)$, we require }
\begin{eqnarray}
    H_{a}^{S_{k}} &=& \frac{\Omega_{a}}{2}(|r_{k-1}\rangle\langle 1_{k-1}|\otimes\mathcal{I}_{k}\otimes\mathcal{I}_{k+1} + \mathcal{I}_{k-1}\otimes|r_{k}\rangle\langle -_{k}|\otimes\mathcal{I}_{k+1} + \mathcal{I}_{k-1}\otimes\mathcal{I}_{k}\otimes|r_{k+1}\rangle\langle 1_{k+1}|) + {\rm H.c.} + H_{V},\cr\cr
    H_{b}^{S_{k}}(t) &=& \frac{\Omega_{b}}{2}e^{i\Delta t}(|r_{k-1}\rangle\langle 1_{k-1}|\otimes\mathcal{I}_{k}\otimes\mathcal{I}_{k+1} + \mathcal{I}_{k-1}\otimes|r_{k}\rangle\langle -_{k}|\otimes\mathcal{I}_{k+1} + \mathcal{I}_{k-1}\otimes\mathcal{I}_{k}\otimes|r_{k+1}\rangle\langle 1_{k+1}|) + {\rm H.c.} + H_{V}.\nonumber
\end{eqnarray}
The effective Zeno Hamiltonian can be obtained as
\begin{equation}\label{eq:H_Sk}
    H_{S_{k}} = \frac{\Omega_\text{eff}}{2}(|r_{k-1}+_{k}0_{k+1}\rangle\langle 1_{k-1}+_{k}0_{k+1}| + |0_{k-1}r_{k}0_{k+1}\rangle\langle 0_{k-1}-_{k}0_{k+1}| + |0_{k-1}+_{k}r_{k+1}\rangle\langle 0_{k-1}+_{k}1_{k+1}|) + {\rm H.c.}
\end{equation}
%%%%  这些有效要不要画一个和原始的对比

\subsection{Explanation of the avoided-crossing phenomenon}

\begin{figure}
	\centering
	\includegraphics[width=18cm]{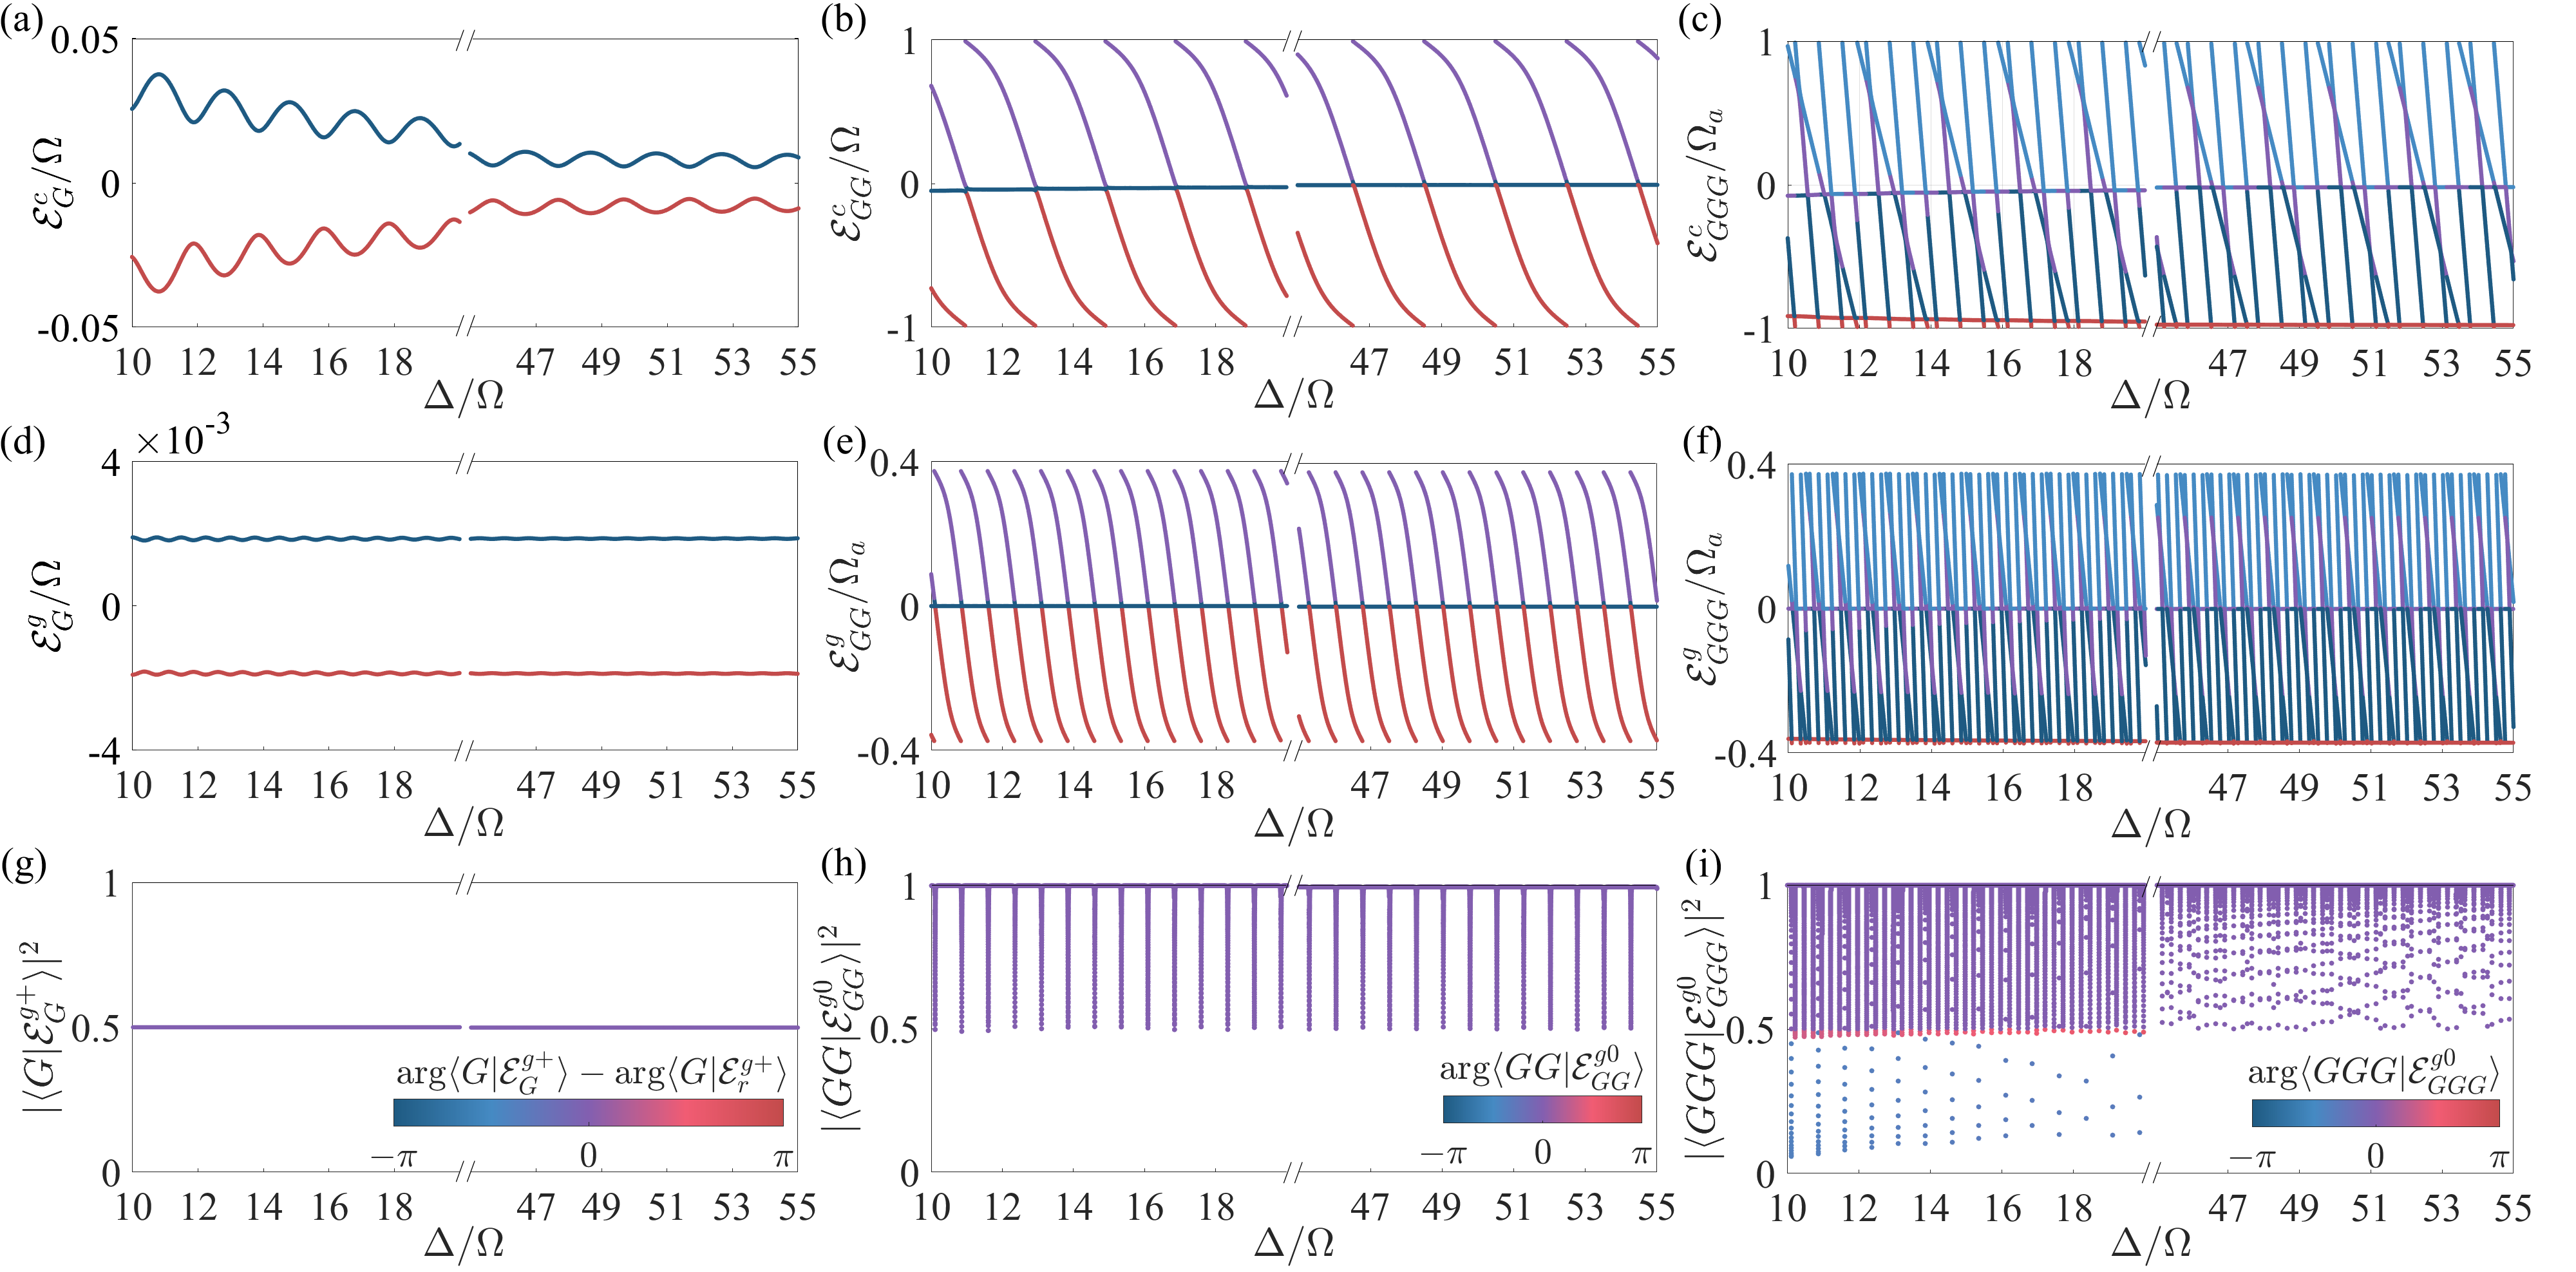}
	\caption{Quasienergy spectra of the Floquet Hamiltonian $H_F$ for single-, two-, and three-atom systems under the Constant-drive scheme (a--c) and the Gaussian-pulse scheme (d--f), plotted as a function of $\Delta/\Omega$. Panels (d), (e), and (f) additionally show the projections of the quantum states of interest onto the corresponding eigenstates in the Gaussian cases. Parameters are set as $\Omega_{a} = \Omega_{b} = \Omega$ for the Constant-drive scheme, and $\Omega_{a} = \max[\Omega_{b}] = \Omega$, $\alpha = 0.6$ for the Gaussian-pulse scheme, and both have $\mathcal{N} = 100$.
}\label{fig_SM_Gaussian}
\end{figure}

The above approximation fails when near degeneracy between the quasienergies of $U_{b}$ leads to strong mixing between system states, a phenomenon displayed as an avoided crossing in the main text. The precise but difficult to analyze result can be given by the Floquet Hamiltonian $H_F = i/T\log[U_b(t_b)U_a(t_a)]$. We simulate numerically the corresponding quasienergy spectra in Figs.~\ref{fig_SM_Gaussian}(a)-(c) for the Hamiltonian in the single-, two-, and three-atom ground state subspaces, where the oscillation in the single-atom ground state case stems from the Stark shifts of Hamiltonian $H_{b_{1}}$ while avoided crossings (corresponding to peaks appearing in the overlap of eigenstates) appear periodically in the quasienergy spectrum. 
% It can be immediately pointed out that the Hamiltonians $H_{b_{2(3)}}$ cause the eigenenergy spectra to rapidly change with detuning $\Delta$, resulting in avoided crossing when near degeneracy occurs between different eigenvalues ($H_{a_{2(3)}}$ are constant Hamiltonians, and the execution time is very short each time, which mainly contribute to the avoided crossing phenomenon by prolonging the cycle time).
Since \(H_a\) acts only for a short duration within each driving cycle, its contribution to the Floquet quasienergy spectrum is limited to a slight modification of the effective period. The dominant role is instead played by \(H_b(t)\). In the following, we take \(H_b(t)\) in the two-atom model as an example to analytically elucidate the origin of the avoided crossings.

The time-dependent Hamiltonian $H_{b_{2}}$ can be transformed to a time-independent Hamiltonian $H'_{b_{2}}$ by the rotating frame $R_{b_{2}} = \exp[i\Delta t(|w\rangle\langle w| + 2|rr\rangle\langle rr|)]$
\begin{eqnarray}\label{eq:time-independent Hb2}
    H' _{b_{2}} &=& \frac{\Omega_{b}}{\sqrt{2}}(|w\rangle\langle GG| + |rr\rangle\langle w|)+{\rm H.c.} + \Delta|w\rangle\langle w| + \Delta|rr\rangle\langle rr|,
\end{eqnarray}  
The periodic avoided crossings in the quasienergy spectrum of $U_{b_2}$, are a hallmark feature of its Floquet dynamics. This phenomenon originates from the periodic `phase kick' delivered by the rotating-frame transformation $R_{b_2}(t_b) = \mathrm{diag}(1, e^{i\Delta t_b}, e^{i2\Delta t_b})$ at each stroboscopic evolution time $t_b$. The nature of the resulting interference is critically dictated by the phase $\phi = \Delta \cdot t_b$ acquired during this period. A strong avoided crossing emerges when this phase kick acts as a symmetry-breaking parity-flip operator, which occurs under the general resonance condition $\Delta \cdot t_b = (2m+1)\pi$ for an integer $m$. Conversely, when the phase kick becomes trivial, it preserves the system's symmetry, which happens when $\Delta \cdot t_b = 2m\pi$. 
%% The scenario presented in Fig.~\ref{fig_SM_constant} (for instance $\Delta/\Omega_{a} = 14$) provides a perfect illustration of this general principle for the specific evolution time $\tau_2 = \pi/\Omega_a$. 
Between them, due to the existence of systemic nonadiabatic transitions, there is also a small mixing between the system states. However, in an ideal situation, this can be avoided by selecting a relatively large detuning.

Furthermore, we provide an analytical argument to demonstrate that under the resonance condition $\Delta \cdot t_b = (2m+1) \pi$, the system is primed to exhibit an avoided-crossing phenomenon.

% --- The Dyson series derivation is well-structured and kept as is ---
The block matrix describing the high-energy subspace $\{|w\rangle, |rr\rangle\}$ within the time-independent Hamiltonian~(\ref{eq:time-independent Hb2}) is
\begin{equation}\label{eq:HD2}
    H'_D = 
    \begin{pmatrix} 
        \Delta & \frac{\Omega_{b}}{\sqrt{2}} \\ 
        \frac{\Omega_{b}}{\sqrt{2}} & \Delta 
    \end{pmatrix},
\end{equation}
which can be diagonalized to yield eigenvalues $E_{\pm} = \Delta \pm \Omega_{b}/\sqrt{2}$ and eigenstates $|E_{\pm}\rangle = 1/\sqrt{2}(|w\rangle \pm |rr\rangle)$.
We can thus rewrite $H'_{b_{2}}$ in the basis $\{|GG\rangle, |E_+\rangle, |E_-\rangle\}$ as
\begin{equation}
    H'_{S} = \underbrace{\begin{pmatrix} 
        0 & 0 & 0 \\ 
        0 & E_+ & 0 \\ 
        0 & 0 & E_- 
    \end{pmatrix}}_{H_0}
    +
    \underbrace{\begin{pmatrix} 
        0 & \frac{\Omega_{b}}{\sqrt{2}} & \frac{\Omega_{b}}{\sqrt{2}} \\ 
        \frac{\Omega_{b}}{\sqrt{2}} & 0 & 0 \\ 
        \frac{\Omega_{b}}{\sqrt{2}} & 0 & 0 
    \end{pmatrix}}_{V'}.
\end{equation}
The transition probability amplitudes for the evolution operator $U_S(t) = \exp(-iH'_S t)$ can be approximated using a Dyson series expansion, since we always assume $\Delta\gg \Omega_b$. To first order, the transition from state $|GG\rangle$ to $|E_{\pm}\rangle$ is given by
\begin{align}
    U_{\pm,GG} &\approx -i \int_0^t e^{iE_\pm t'} \langle E_\pm | V' | GG \rangle dt' = -\frac{\Omega_{b}}{\sqrt{2}} \frac{e^{iE_\pm t} - 1}{E_\pm}.
\end{align}
Transforming back to the $\{|w\rangle, |rr\rangle\}$ basis, we obtain the off-diagonal elements
\begin{align}
    U_{w,GG} &= \frac{1}{\sqrt{2}} [U_{+,GG}(t) + U_{-,GG}(t)] \approx -\frac{\Omega_{b}}{2} \left( \frac{e^{iE_+ t} - 1}{E_+} + \frac{e^{iE_- t} - 1}{E_-} \right), \\
    U_{rr,GG} &= \frac{1}{\sqrt{2}} [U_{+,GG}(t) - U_{-,GG}(t)] \approx -\frac{\Omega_{b}}{2} \left( \frac{e^{iE_+ t} - 1}{E_+} - \frac{e^{iE_- t} - 1}{E_-} \right).
\end{align}
To zeroth order, the elements within the high-energy subspace are
\begin{align}
    U_{w,w} &\approx \frac{1}{2}(e^{-iE_+ t} + e^{-iE_- t}), \quad U_{rr,rr} \approx \frac{1}{2}(e^{-iE_+ t} + e^{-iE_- t}),\\
    U_{w,rr} &\approx \frac{1}{2}(e^{-iE_+ t} - e^{-iE_- t}), \quad U_{rr,w} \approx \frac{1}{2}(e^{-iE_+ t} - e^{-iE_- t}).
\end{align}
Meanwhile, the diagonal element $U_{GG,GG}(t)$ is calculated to second order:
\begin{eqnarray}
    U_{GG,GG} \approx 1 + U^{(2)}_{GG,GG}(t),
\end{eqnarray}
with 
\begin{eqnarray}
    U^{(2)}_{GG,GG} &=& -\sum_{k \in \{+,-\}} \int_0^t dt_1 \int_0^{t_1} dt_2 \langle GG|V' e^{-iE_k(t_1-t_2)}V'|GG\rangle\cr\cr
    &=& i\frac{\Omega_{b}^2}{2} t \left( \frac{1}{E_+} + \frac{1}{E_-} \right) - \frac{\Omega_{b}^2}{2} \left( \frac{1 - e^{-iE_+ t}}{E_+^2} + \frac{1 - e^{-iE_- t}}{E_-^2} \right).
\end{eqnarray}

The full evolution operator for the kick Hamiltonian is then constructed by applying the rotating-frame transformation
\begin{eqnarray}
    U_{b_{2}}(t) &\approx& R_{b_{2}}(t) U'_{b_{2}}(t) \cr\cr
    &=& \begin{pmatrix} 
        1 & 0 & 0 \\ 
        0 & e^{i \Delta t} & 0\\
        0 & 0 & e^{2 i \Delta t}  % Note: Paper has a small typo here, should be 2*Delta*t for |rr>
    \end{pmatrix}
    \begin{pmatrix} 
        U_{GG,GG} & U_{GG,w} & U_{GG,rr} \\ 
        U_{w,GG} & U_{w,w} & U_{w,rr}\\
        U_{rr,GG} & U_{rr,w} & U_{rr,rr}
    \end{pmatrix}.
\end{eqnarray}
Focusing on the high-energy subspace, its dynamics are governed by the effective block matrix $U_{D}$:
\begin{eqnarray}
    U_{D}(t) = \begin{pmatrix} 
        e^{i\Delta t}U_{w,w} & e^{i\Delta t}U_{w,rr} \\
        e^{2i\Delta t}U_{rr,w} & e^{2i\Delta t}U_{rr,rr}
    \end{pmatrix}
    \approx
    \begin{pmatrix} 
        \cos(\frac{\Omega_{b}}{\sqrt{2}} t) & -i \sin(\frac{\Omega_{b}}{\sqrt{2}} t)\\
        -i e^{i \Delta t}\sin(\frac{\Omega_{b}}{\sqrt{2}}t) & e^{i \Delta t}\cos(\frac{\Omega_{b}}{\sqrt{2}}t)
    \end{pmatrix}.
\end{eqnarray}
This brings us to the core of the argument. Under the resonance condition $\Delta \cdot t = (2m+1)\pi$, the matrix $U_D$ simplifies and yields eigenvalues of $\pm 1$. The corresponding normalized eigenstates are $|v_1\rangle = -i\cos[(2m+1)\pi\Omega_b /(2\sqrt{2}\Delta)]|w\rangle + \sin[(2m+1)\pi\Omega_b /(2\sqrt{2}\Delta)]|rr\rangle$ for the eigenvalue $+1$, and $|v_2\rangle = i\sin[(2m+1)\pi\Omega_b /(2\sqrt{2}\Delta)]|w\rangle + \cos[(2m+1)\pi\Omega_b /(2\sqrt{2}\Delta)]|rr\rangle$ for the eigenvalue $-1$.

The eigenvalue of $+1$ is of critical importance, as it corresponds to a quasienergy of $\epsilon = 0$ (within the first Brillouin zone). The low-energy ground state $|GG\rangle$ also has a quasienergy approximately equal to zero. Therefore, the resonance condition creates a quasienergy degeneracy: an effective mode from the high-energy subspace, $|v_1\rangle$, has nearly the same quasienergy as the ground state. The coupling induces a repulsion between the quasienergy levels, preventing them from crossing, i.e., avoided crossing, which facilitates strong state mixing and resonant population transfer, perfectly explaining the sharp spikes observed in the simulations.

The similar result also appears in the three-atom ground state Hamiltonian $H_{b_3}$. It can be transformed into 
\begin{eqnarray}\label{eq:time-independent Hb3}
    H'_{b_{3}} &=& \frac{\Omega_{b}}{2}(\sqrt{3}|w_1\rangle\langle GGG| + 2| w_2\rangle\langle w_1| + \sqrt{3}|rrr\rangle\langle w_2|) + {\rm H.c.} + \Delta|w_1\rangle\langle w_1| + \Delta|w_2\rangle\langle w_2|.
\end{eqnarray}
by a rotation transform $R_{b_3} = \exp[i\Delta t (|w_1\rangle\langle w_1| + 2|w_2\rangle\langle w_2| + 3|rrr\rangle\langle rrr|)]$.

At this point, the block matrix describing the high-energy subspace 
$\{|w_1\rangle, |w_2\rangle\}$ within the time-independent Hamiltonian~(\ref{eq:time-independent Hb3}) 
takes a form similar to that of Eq.~(\ref{eq:HD2}). 
Owing to the fact that the corresponding rotation matrix $R_{b_3}$ now contains 
a detuning that is three times larger, the quasienergy spectrum exhibits 
not only the same avoided-crossing period as in the two-atom case, 
but also an additional smaller period equal to one third of the 
two-atom avoided-crossing period.

\subsection{Optimization of the scheme}

% While the proposed bang-bang scheme is theoretically feasible,  its practical implementation requires addressing several key experimental challenges.

Figure~\ref{fig_SM_Gaussian}(a) shows a very obvious oscillation of the quasienergy spectra of a single-atom ground state subsystem, which would be reflected in the significant changes observed in state evolution with detuning $\Delta$. Additionally, Figs.~\ref{fig_SM_Gaussian}(b) and (c) demonstrate that the quasienergy of the ground states $|GG\rangle$ and $|GGG\rangle$ cannot strictly approach 0.

Therefore, we propose implementing the kick drive not with square pulses, but with smooth Gaussian pulses. This approach offers enhanced robustness against parameter noise. The pulse shape is defined as: 
\begin{equation}
    \Omega_{b}(t) = \Omega\exp\left[-\frac{(t-2t_{f})^2}{2(\alpha t_{f})^2}\right],
\end{equation}
where \(\Omega\) is the peak amplitude, the total pulse duration is \(t_b = 4t_{f}\), and \(t_f\) is related to the pulse area by \(t_f = \sqrt{\pi/2}/[\alpha \Omega {\rm Erf}(\sqrt{2}/\alpha)]\).
 Additionally, to resist Stark shifts from the kick Hamiltonian, we introduce another laser beam with opposite detuning. The new kick Hamiltonian can be expressed as
\begin{equation}
    H_{b}(t) = \sum_{i}\frac{\Omega_{b}(t)}{2}(e^{-i\Delta t} + e^{i\Delta t})|r_{i}\rangle\langle G_{i}| + {\rm H.c.} + H_{V} = \sum_{i}\Omega_{b}\cos(\Delta t)|r_{i}\rangle\langle G_{i}| + {\rm H.c.} + H_{V}.
    \label{eq:remove_stark_shift}
\end{equation}
To demonstrate the performance of the proposed optimization, we numerically demonstrate the quasienergy spectra under the Gaussian scheme shown in Figs.~\ref{fig_SM_Gaussian}(d)-(f). Compared to the Constant scheme in Figs.~\ref{fig_SM_Gaussian}(a)-(c), the Gaussian one demonstrates an approximate flat band in the single-atom case and has quasienergy closer to 0 in the two- and three-atom cases. We also point out that due to the longer time required for the Gaussian pulse to obtain the same pulse area as the Constant scheme, the corresponding avoided-crossing frequency is reduced, resulting in more avoided-crossing positions compared to the Constant scheme. Finally, we display the projection of the quantum states of interest onto the corresponding eigenstates under the Gaussian case in Figs.~\ref{fig_SM_Gaussian}(g)-(i), where strong state mixing occurs in the avoided-crossing position, and the ground state components of the eigenstates undergo rapid changes.

\section{Engineering dissipation of Rydberg state}\label{Appendix_B}

The lifetime of the Rydberg state $|r\rangle$ is often in the millisecond range, much longer than that of intermediate low excited state $\ket{p}$, even nanoseconds. For simplicity, we neglect the spontaneous emission rate $\gamma_{r}$ of the Rydberg state at this stage.
 Besides, the intermediate state is assumed to decay only into the sector $|0\rangle$ due to the selection rule (this can be realized by choosing the stretched $nP$ states, for example, $|p\rangle \equiv |5P_{3/2}, F=3, m_{F}=3\rangle$ with a lifetime $\tau_{p} = 1/\gamma_{p} = 26.2$ ns). Utilizing an additional laser to drive resonantly $|r \rangle \stackrel{\Omega_{p}}{\longleftrightarrow} |p\rangle$, we can realize the effective dissipation to the ground state $|0\rangle$.

\begin{figure}
	\centering
	\includegraphics[width=1\linewidth]{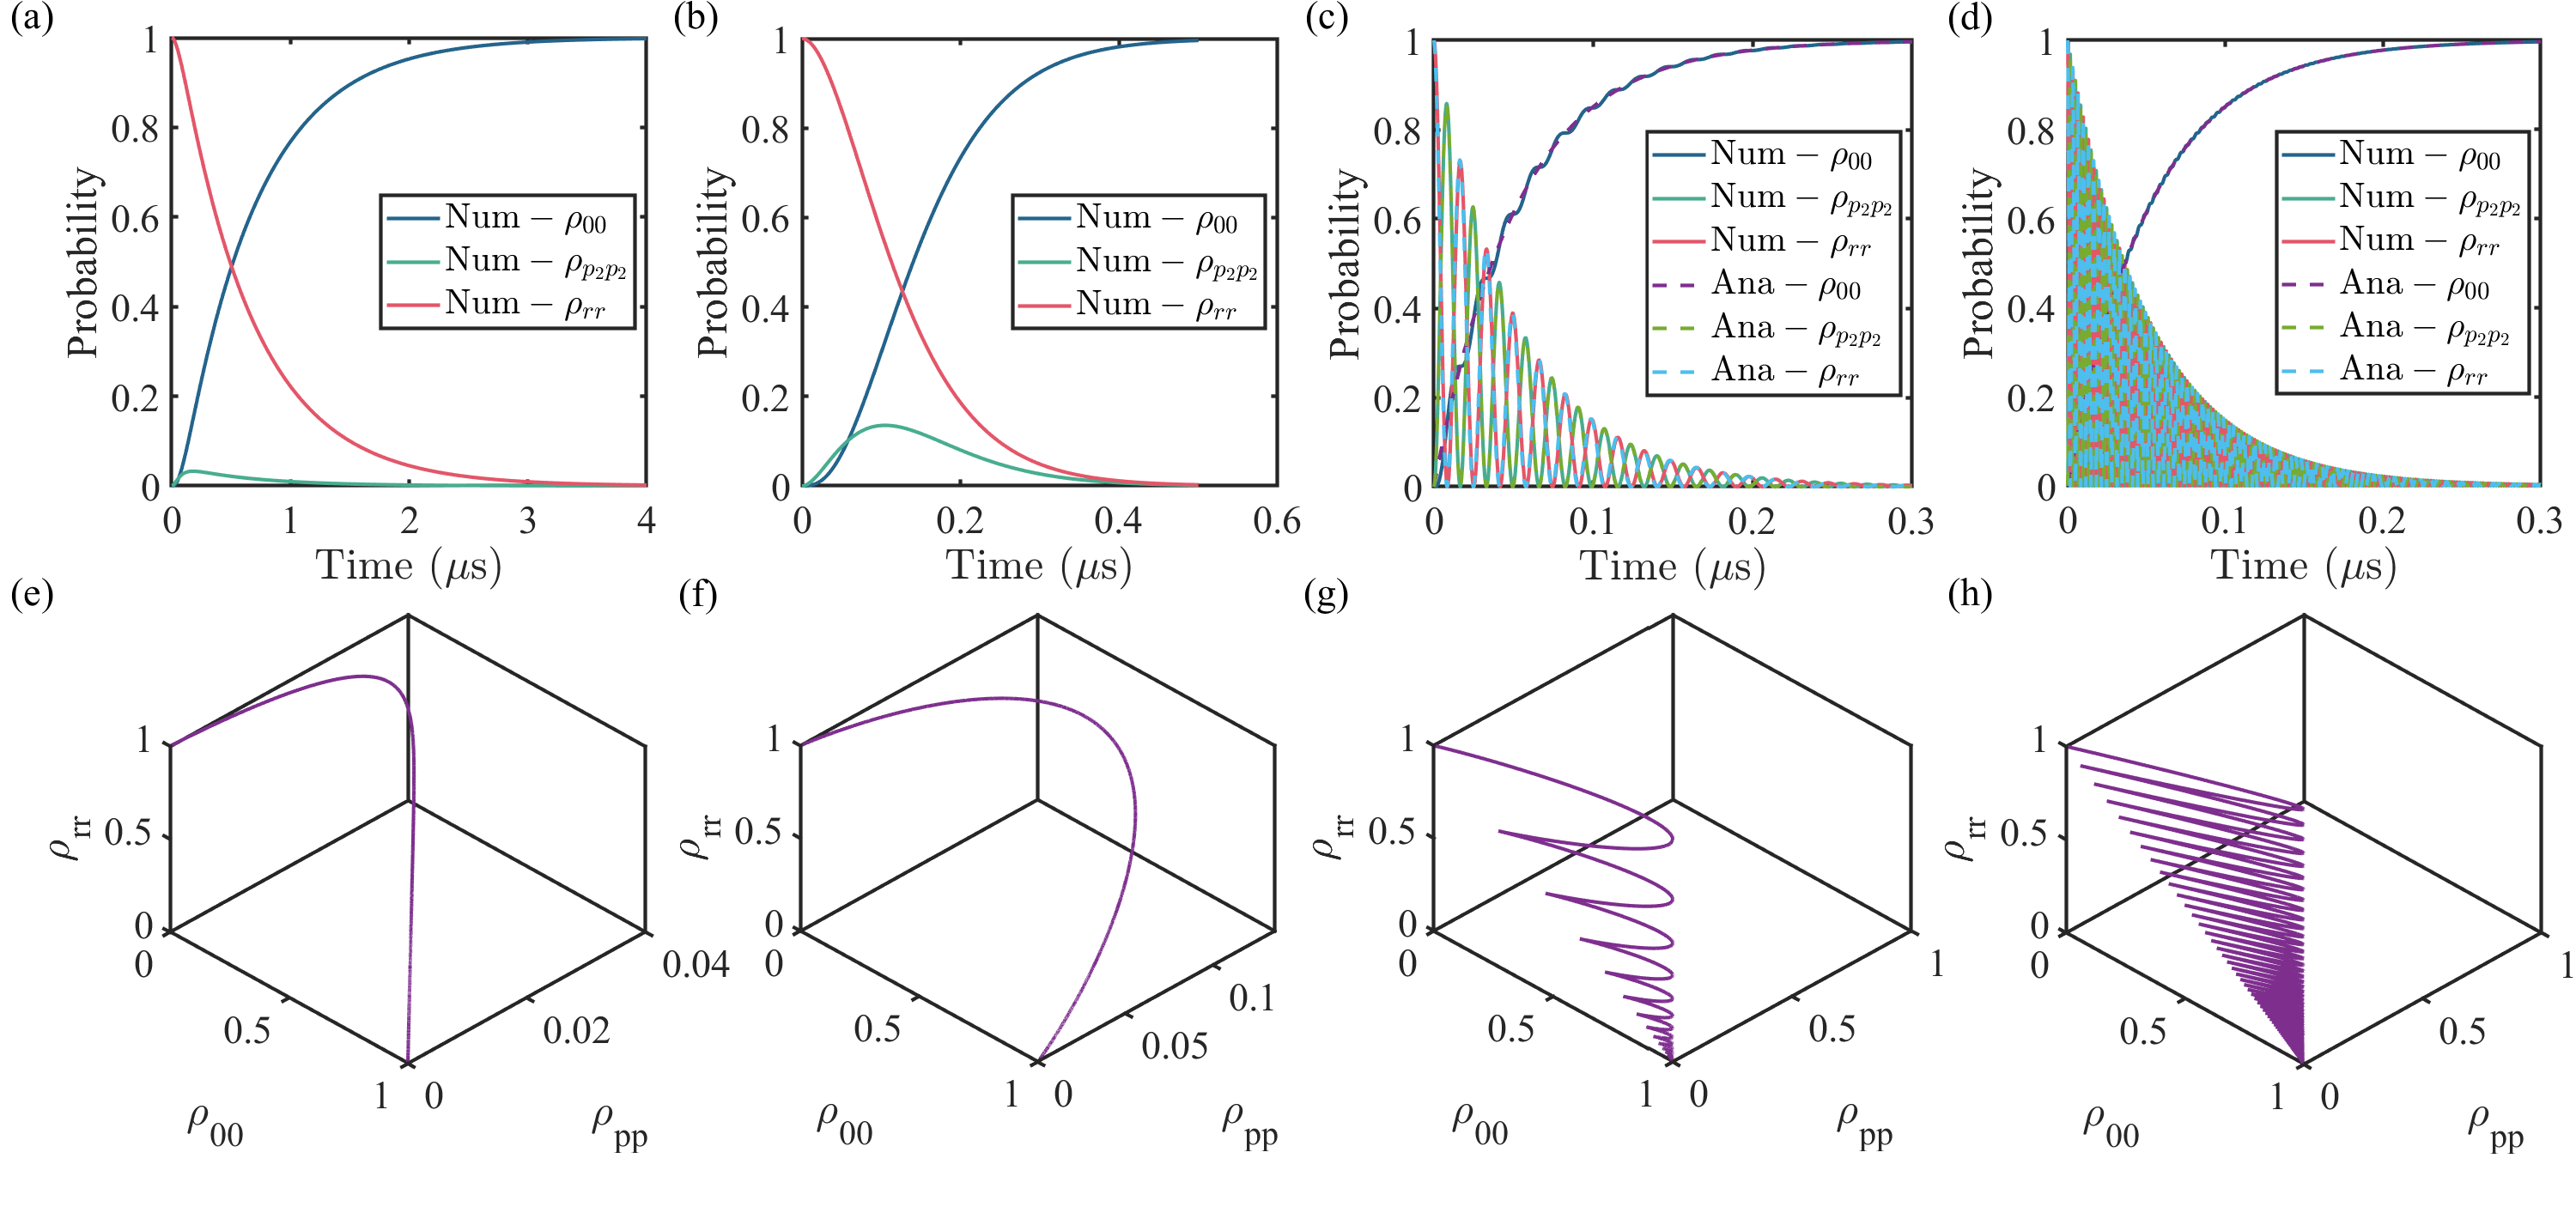}
	\caption{Probabilities of $\rho_{00}$, $\rho_{pp}$, $\rho_{rr}$ for the conditions (a) $\Omega_{p} = 0.2\gamma_{p}$; (b) $\Omega_{p} = 0.5\gamma_{p}$; (c) $\Omega_{p} = 10\gamma_{p}$; (a) $\Omega_{p} = 50\gamma_{p}$ considering numerical analyses. (c) and (d) additionally consider analytical solutions in Eq.~(\ref{fig_outweigh}) when $\Omega_{p}\gg \gamma_{p}$, showing almost consistency between numerical and analysis results. (e)-(h) show the relaxation process for three states $\rho_{00}$, $\rho_{pp}$, $\rho_{rr}$ denoted by probabilities, ultimately reaching stability.}\label{fig_relaxation}
\end{figure}

%%% 还想额外加一点关于mpemba效应中 C1（对应λ1本征值）系数的讨论

From the perspective of Liouvillian space, the eigenenergy spectrum 
%%$g = \min\{{\rm Re}[E_{i}|_{E_{i}\neq 0}]\}$
%%with $E_{i}$ being the $i$th eigenvalue of Liouvillian superoperator in Eq.~(\ref{eq_liouvillian})
determines the timescale of system relaxation to stationarity~\cite{Carollo2021Exponentially, Zhou2023Accelerating}. This can be used to modulate the relaxation time (for instance, by tuning the initial subspace, the convergence speed can be effectively controlled, showcasing the Mpemba effect). Reference~\cite{Zhou2023Accelerating} showcases that there exists a faster relaxation rate in the entire system space when the slowest decay mode degenerates with a faster decay mode. Considering the driven $H_{rp} = \Omega_{p}/2|r\rangle\langle p| + {\rm H.c.}$, the Liouvillian superoperator can be expressed as
\begin{eqnarray}
    \hat{\mathcal{L}}_{d} = -i(H_{rp}\otimes \mathcal{I} - \mathcal{I}\otimes H_{rp}^{\rm T}) + L_{0p}\otimes L_{0p}^{*} - \frac{1}{2}(L_{0p}^{\dagger}L_{0p}\otimes \mathcal{I} + \mathcal{I} \otimes L_{0p}^{\rm T}L_{0p}^{*})
\end{eqnarray}
with $L_{0p} = \sqrt{\gamma_{p}}|0\rangle\langle p|$. The eigenvalues are 
\[\lambda_{0} = 0,~~~\lambda_{1,2} = -(\gamma_{p} - \kappa)/4,~~~\lambda_{3,4} = -(\gamma_{p} + \kappa)/4,~~~\lambda_{5} = -(\gamma_{p} - \kappa)/2,~~~\lambda_{6,7} = -\gamma_{p}/2,~~~\lambda_{8} = -(\gamma_{p} + \kappa)/2\]
with $\kappa = \sqrt{\gamma_{p}^2 - 4\Omega_{p}^2}$, and the corresponding right and left eigenmatrices are ($|0\rangle \equiv (1~0~0)^{T}$, $|p\rangle \equiv (0~1~0)^{T}$, and $|r\rangle \equiv (0~0~1)^{T}$)
\begin{align}
r_0 &= \begin{pmatrix} 1 & 0 & 0 \\ 0 & 0 & 0 \\ 0 & 0 & 0 \end{pmatrix}, \quad
r_1 = \frac{1}{N_{-}} \begin{pmatrix} 0 & 0 & 0 \\ -i (\gmp - \kpp) & 0 & 0 \\ 2 \omp & 0 & 0 \end{pmatrix}, \quad
r_2 = \frac{1}{N_{-}} \begin{pmatrix} 0 & i (\gmp - \kpp) & 2 \omp \\ 0 & 0 & 0 \\ 0 & 0 & 0 \end{pmatrix}, \cr\cr
r_3 &= \frac{1}{N_{+}} \begin{pmatrix} 0 & 0 & 0 \\ -i (\gmp + \kpp) & 0 & 0 \\ 2 \omp & 0 & 0 \end{pmatrix}, \quad
r_4 = \frac{1}{N_{+}} \begin{pmatrix} 0 & i (\gmp + \kpp) & 2 \omp \\ 0 & 0 & 0 \\ 0 & 0 & 0 \end{pmatrix}, \quad
r_5 = \begin{pmatrix} -\frac{\gmp (\gmp - \kpp)}{2 \omp^2} & 0 & 0 \\ 0 & 1 - \frac{\kpp (\gmp - \kpp)}{2 \omp^2} & -\frac{i (\gmp - \kpp)}{2 \omp} \\ 0 & \frac{i (\gmp - \kpp)}{2 \omp} & 1 \end{pmatrix}, \cr\cr
r_6 &= \frac{\sqrt{2}}{D_0} \begin{pmatrix} -2 \omp & 0 & 0 \\ 0 & \omp & -i \gmp/2 \\ 0 & i \gmp/2 & \omp \end{pmatrix}, \quad
r_7 = \frac{1}{\sqrt{2}} \begin{pmatrix} 0 & 0 & 0 \\ 0 & 0 & 1 \\ 0 & 1 & 0 \end{pmatrix}, \quad
r_8 = \begin{pmatrix} -\frac{\gmp (\gmp + \kpp)}{2 \omp^2} & 0 & 0 \\ 0 & -1 + \frac{\gmp (\gmp + \kpp)}{2 \omp^2} & -\frac{i (\gmp + \kpp)}{2 \omp} \\ 0 & \frac{i (\gmp + \kpp)}{2 \omp} & 1 \end{pmatrix},\nonumber
\end{align}
and
\begin{align}
l_0^{\dagger} &= \begin{pmatrix} 1 & 0 & 0 \\ 0 & 1 & 0 \\ 0 & 0 & 1 \end{pmatrix}, \quad
l_1^{\dagger} = \frac{N_{-}}{4\omp|\kpp|} \begin{pmatrix} 0 & 0 & 0 \\ 2i\omp & 0 & 0 \\ \gmp + \kpp & 0 & 0 \end{pmatrix}, \quad
l_2^{\dagger} = \frac{N_{-}}{4\omp|\kpp|} \begin{pmatrix} 0 & -2i\omp & \gmp + \kpp^* \\ 0 & 0 & 0 \\ 0 & 0 & 0 \end{pmatrix}, \cr\cr
l_3^{\dagger} &= \frac{N_{+}}{4\omp|\kpp|} \begin{pmatrix} 0 & 0 & 0 \\ -2i\omp & 0 & 0 \\ -\gmp + \kpp^* & 0 & 0 \end{pmatrix}, \quad
l_4^{\dagger} = \frac{N_{+}}{4\omp|\kpp|} \begin{pmatrix} 0 & 2i\omp & -\gmp + \kpp^* \\ 0 & 0 & 0 \\ 0 & 0 & 0 \end{pmatrix}, \quad
l_5^{\dagger} = D_{-}
\begin{pmatrix}
0 & 0 & 0 \\
0 & \frac{P_0 \kappa^* + Q_0}{\Omega_p^2} & \frac{P_{pr} + Q_{pr}}{\Omega_p^3} \\
0 & -\frac{P_{pr} + Q_{pr}}{\Omega_p^3} & \frac{P_{rr} + Q_{rr}}{\Omega_p^4}
\end{pmatrix}, \cr\cr
l_6^{\dagger} &= -\frac{\sqrt{2}D_0}{\kpp^2} \begin{pmatrix} 0 & 0 & 0 \\ 0 & \omp & i\gmp/2 \\ 0 & -i\gmp/2 & \omp \end{pmatrix}, \quad
l_7^{\dagger} = \frac{1}{\sqrt{2}} \begin{pmatrix} 0 & 0 & 0 \\ 0 & 0 & 1 \\ 0 & 1 & 0 \end{pmatrix}, \quad
l_8^{\dagger} = D_{+}
\begin{pmatrix}
0 & 0 & 0 \\
0 & \frac{P_0 \kappa^* - Q_0}{\Omega_p^2} & -\frac{P_{pr} - Q_{pr}}{\Omega_p^3} \\
0 & \frac{P_{pr} - Q_{pr}}{\Omega_p^3} & \frac{P_{rr} - Q_{rr}}{\Omega_p^4}
\end{pmatrix},\nonumber
\end{align}
with
\begin{align}
    N_{\pm} &= \sqrt{4\omp^2 + |\gmp \pm \kpp|^2}, \quad
    D_0 = \sqrt{16\omp^2 + \kpp^2}, \quad
    P_0 = 2\kappa^2 + 5\Omega_p^2, \quad
    Q_0 = \gamma_p(2\kappa^2 + \Omega_p^2), \cr\cr
    P_{pr} &= i(2\kappa^4 + 7\kappa^2\Omega_p^2 + 2\Omega_p^4), \quad
    Q_{pr} = i\gamma_p(2\kappa^2 + 3\Omega_p^2)\kappa^*, \quad
    P_{rr} = (\kappa^2 + \Omega_p^2)(2\kappa^2 + 7\Omega_p^2)\kappa^*, \cr\cr
    Q_{rr} &= \gamma_p(2\kappa^4 + 5\kappa^2\Omega_p^2 + \Omega_p^4), \quad
    D_1 = 4\kappa^2(2\kappa^2 - \Omega_p^2)\kappa^*, \quad
    D_{\pm} = (\kappa^2 P_0 \pm Q_0 \kappa^*)/D_1. \nonumber
\end{align}

This system exists a third-order ($\lambda_{5} = \lambda_{6} = \lambda_{8}, r_{5} = r_{6} = r_{8}$ up to a normalization factor) and two second-order LEPs ($\lambda_{1} = \lambda_{3}, r_{1} = r_{3}$ and $\lambda_{2} = \lambda_{4}, r_{2} = r_{4}$) when $\Omega_{p} = 0.5\gamma_{p}$.

%%%%%%%%% 这里考虑把本征态也加上，表示由于r态的选择本身的衰减速率就是-gamma/2

Here we propose another acceleration method requiring $\Omega_{p} > 0.5\gamma_{p}$ when placing the perspective on the accumulation of steady state $\rho_{ss}$. As shown in Fig~\ref{fig_relaxation}, it showcases the system converges faster and faster as $\Omega_p$ becomes larger than $\gamma_p$, and reaches a stable convergence ($\Omega_{p} \gg \gamma_{p}$) with a maximum relaxation rate of $\gamma_{p}/2$. Next, we provide an analytical process. 

Assume the initial state $\rho(0) = \rho_{rr}$, we thus have ${\rm Tr}[l_{1-4}\rho_{rr}]={\rm Tr}[l_{7}\rho_{rr}]=0$. 
This indicates that a specific initial state $\rho_{rr}$ determines the minimum convergence speed of the system guided by $\lambda_{5}$. We thus reduce the evolution state into the time-dependent density matrix 
\begin{eqnarray}
    \rho(t) &=& r_{0} + c_{5}(t)r_{5} + c_{6}(t)r_{6} + c_{8}(t)r_{8}\cr\cr
    &=& r_{0} + \frac{\kappa (\gamma_{p} + \kappa) + 2 \Omega_{p}^2}{2 \kappa^2}e^{\lambda_{5}t} r_{5} - \frac{\sqrt{2} \Omega_{p} \sqrt{16 \Omega_{p}^2 + \kappa^2}}{\kappa^2}e^{\lambda_{6}t} r_{6} + \frac{\kappa (\kappa - \gamma_{p}) + 2 \Omega_{p}^2}{2 \kappa^2}e^{\lambda_{8}t} r_{8} \cr\cr
    &=& \left\{1 + \frac{e^{-\frac{\gamma_{p}t}{2}} \left[ 4 \Omega_{p}^2 - \left( \kappa^2 + 4 \Omega_{p}^2 \right) \cosh\left( \frac{t \kappa}{2} \right) - \gamma_{p} \kappa \sinh\left( \frac{t \kappa}{2} \right) \right]}{\kappa^2}\right\}|0\rangle\langle 0|
    + \frac{4 e^{-\frac{\gamma_{p}t}{2}} \Omega_{p}^2 \sinh^2\left( \frac{t \kappa}{4} \right)}{\kappa^2}|p\rangle\langle p|\cr\cr
    &&- \frac{i e^{-\frac{\gamma_{p}t}{2}} \Omega_{p} \left[ 2 \gamma_{p} \sinh^2\left( \frac{t \kappa}{4} \right) + \kappa \sinh\left( \frac{t \kappa}{2} \right) \right]}{\kappa^2}|p\rangle\langle r|
    + \frac{i e^{-\frac{\gamma_{p}t}{2}} \Omega_{p} \left[ 2 \gamma_{p} \sinh^2\left( \frac{t \kappa}{4} \right) + \kappa \sinh\left( \frac{t \kappa}{2} \right) \right]}{\kappa^2}|r\rangle\langle p|\cr\cr
    &&+ \frac{e^{-\frac{\gamma_{p}t}{2}} \left[ -2 \Omega_{p}^2 + \left( \kappa^2 + 2 \Omega_{p}^2 \right) \cosh\left( \frac{t \kappa}{2} \right) + \gamma_{p} \kappa \sinh\left( \frac{t \kappa}{2} \right) \right]}{\kappa^2}|r\rangle\langle r|.
\end{eqnarray}

Specifically, we point out that the coherence $\rho_{rp}+\rho_{pr}$ has no contribution to the dynamics. As shown in Figs.~\ref{fig_relaxation}(c) and~\ref{fig_relaxation}(d), this can be numerically simulated to obtain consistent results. We also point out that the convergence of $\rho_{00}(t)$ accelerates with the increase of $\rho_{pp}(t)$ and $\rho_{rr}(t)$ exchange speed, as shown in Figs.~\ref{fig_relaxation}(e)-(h). 
In fact, the $\rho_{00}(t)$ can also be rewritten as
\begin{eqnarray}
    \rho_{00}(t) &=& 1 - \rho_{pp}(t) - \rho_{rr}(t)\cr\cr
    &=& 1 + \frac{e^{-\frac{\gamma_{p}t}{2}} \left[ 4 \Omega_{p}^2 - \left( \kappa^2 + 4 \Omega_{p}^2 \right) \cosh\left( \frac{t \kappa}{2} \right) - \gamma_{p} \kappa \sinh\left( \frac{t \kappa}{2} \right) \right]}{\kappa^2}\cr\cr
    &=& 1 - e^{-\frac{\gamma_{p}t}{2}} + e^{-\frac{\gamma_{p}t}{2}} \cdot \frac{\gamma_{p}^2[1-\cosh(\frac{\kappa t}{2})]-\gamma_{p}\kappa \sinh(\frac{\kappa t}{2})}{\kappa^2}.
\end{eqnarray}

The value of $\kappa^2$ determines three different mechanisms of the system: (i) $\kappa^2>0$ corresponds to an overdamped mechanism. We rewrite
\begin{eqnarray}
    \rho_{00}(t) = 1 - \frac{\gamma_{p}^2+\gamma_{p} \kappa}{2\kappa^2}e^{\lambda_{5}t} - (1-\frac{\gamma_{p}^2}{\kappa^2})e^{\lambda_{6}t} - \frac{\gamma_{p}^2-\gamma_{p} \kappa}{2\kappa^2}e^{\lambda_{8}t},
\end{eqnarray}
It has a slower decay mode $\lambda_{5} = -(\gamma_{p} - \kappa)/2$, a mode $\lambda_{6} = -\gamma_{p}/2$, and a faster decay mode $\lambda_{8} = -(\gamma_{p} + \kappa)/2$. At this point, the convergence speed of the system is mainly determined by the slower mode $\lambda_{5}$. Under extreme conditions $\Omega_{p} \ll \gamma_{p}$ we have further expanded $\Omega_{p}$ to second order 
\begin{eqnarray}
    \rho_{00}(t) \approx 1 - \exp\left({-\frac{\Omega_{p}^2t}{\gamma_{p}}}\right).
\end{eqnarray}
The result is the same as that obtained by employing perturbation theory and adiabatic elimination.

(ii) $\kappa^2=0$ corresponds to a critical damping mechanism. There is no analytical solution for the LEP point, but we can perform an approximate analysis near the LEP point. This can be achieved through the use of the L$^\prime$H$\rm \hat{o}$pital$^\prime$s rule, deriving 
\begin{eqnarray}
    \rho_{00}(t) &=& \lim_{\kappa \to 0} 
    1 - e^{-\frac{\gamma_{p}t}{2}} + e^{-\frac{\gamma_{p}t}{2}} \cdot \frac{\gamma_{p}^2[1-\cosh(\frac{\kappa t}{2})]-\gamma_{p}\kappa \sin(\frac{\kappa t}{2})}{\kappa^2}\cr\cr
    &=& 1-\exp\left[-\frac{\gamma_pt}{2}+\ln\left(1+ \frac{\gamma_{p} t}{2} + \frac{\gamma_{p}^2 t^2}{8}\right)\right].
\end{eqnarray}

(iii) $\kappa^2<0$ corresponds to an underdamped mechanism. Unlike the first two mechanisms, the system will experience strong oscillations and eventually reach an equilibrium state. However, we propose when $\Omega_{p}^2\gg\gamma_{p}$ the system will exhibit an approximate critical damping phenomenon under the underdamped mechanism presented by
\begin{eqnarray}
    \rho_{00}(t) &\approx& 1 -\exp\left({-\frac{\gamma_{p} t}{2}}\right).
\end{eqnarray}
At this point, the system demonstrates a convergence rate faster than the critical damping mechanism. In addition, the effective form of the entire system can be demonstrated as
\begin{eqnarray}\label{fig_outweigh}
    \rho(t) &\approx&
(1 - e^{-\frac{\gamma_{p} t}{2}})|0\rangle\langle 0|
+ \frac{1 - \cos (\Omega_{p} t)}{2}e^{-\frac{\gamma_{p} t}{2}} |p\rangle\langle p|
+ \frac{i \sin (\Omega_{p} t)}{2} e^{-\frac{\gamma_{p} t}{2}} |p\rangle\langle r|
\cr\cr
&&-\frac{i \sin (\Omega_{p} t)}{2} e^{-\frac{\gamma_{p} t}{2}}|r\rangle\langle p|
+ \frac{1 + \cos (\Omega_{p} t)}{2}e^{-\frac{\gamma_{p} t}{2}}|r\rangle\langle r|.
\end{eqnarray}
Meanwhile, it can be observed that the evolution of the states $|p\rangle$ and $|r\rangle$ still maintains high-speed oscillations with $\Omega_{p}$ as the frequency.

\section{The effect of the spontaneous emission from the state $|r\rangle$}\label{sec_steady}

In both the main text and the previous section, we ignore the spontaneous emission from the Rydberg state $\ket{r}$ because the Rabi frequency is in the megahertz range, while the dissipation rate of the Rydberg state is in the kilohertz range. While this assumption has minimal impact on the engineered dissipation, its influence on the excitation process must be carefully examined, especially since the primary duration of the scheme is spent on coherently pumping out unwanted components. Here, taking the Bell state as an example, we show through numerical simulation 
that the spontaneous emission of the Rydberg state has a negligible effect.
The system dynamics are described by the Lindblad master equation:\begin{eqnarray}
   \dot{\rho}(t) = \mathcal{\hat{L}}[\rho(t)]
   = -i[H_{\rm total}(t),\rho(t)] + \sum_{k=0,1}\sum_{n=1,2} L_{kr}^{(n)}\rho(t) L_{kr}^{(n)^\dagger} - \frac{1}{2}\{L_{kr}^{(n)^\dagger}L_{kr}^{(n)}, \rho(t)\},\nonumber
\end{eqnarray}
where $L_{kr}^{(n)} = \sqrt{\gamma_{r}/2}\ket{k_{n}}\bra{r_{n}}$ with the decay rate $\gamma_{r}/(2\pi) = 0.313$~kHz. 
As shown in Fig.~\ref{fig_VS_decay_r}, the inclusion of the spontaneous decay from the Rydberg state to the ground qubit states does not compromise the success of the scheme. The insert highlights the fidelity in the final time interval, demonstrating that the impact of the spontaneous emission is negligible under the given parameters.

\begin{figure}
	\centering
	\includegraphics[width=10cm]{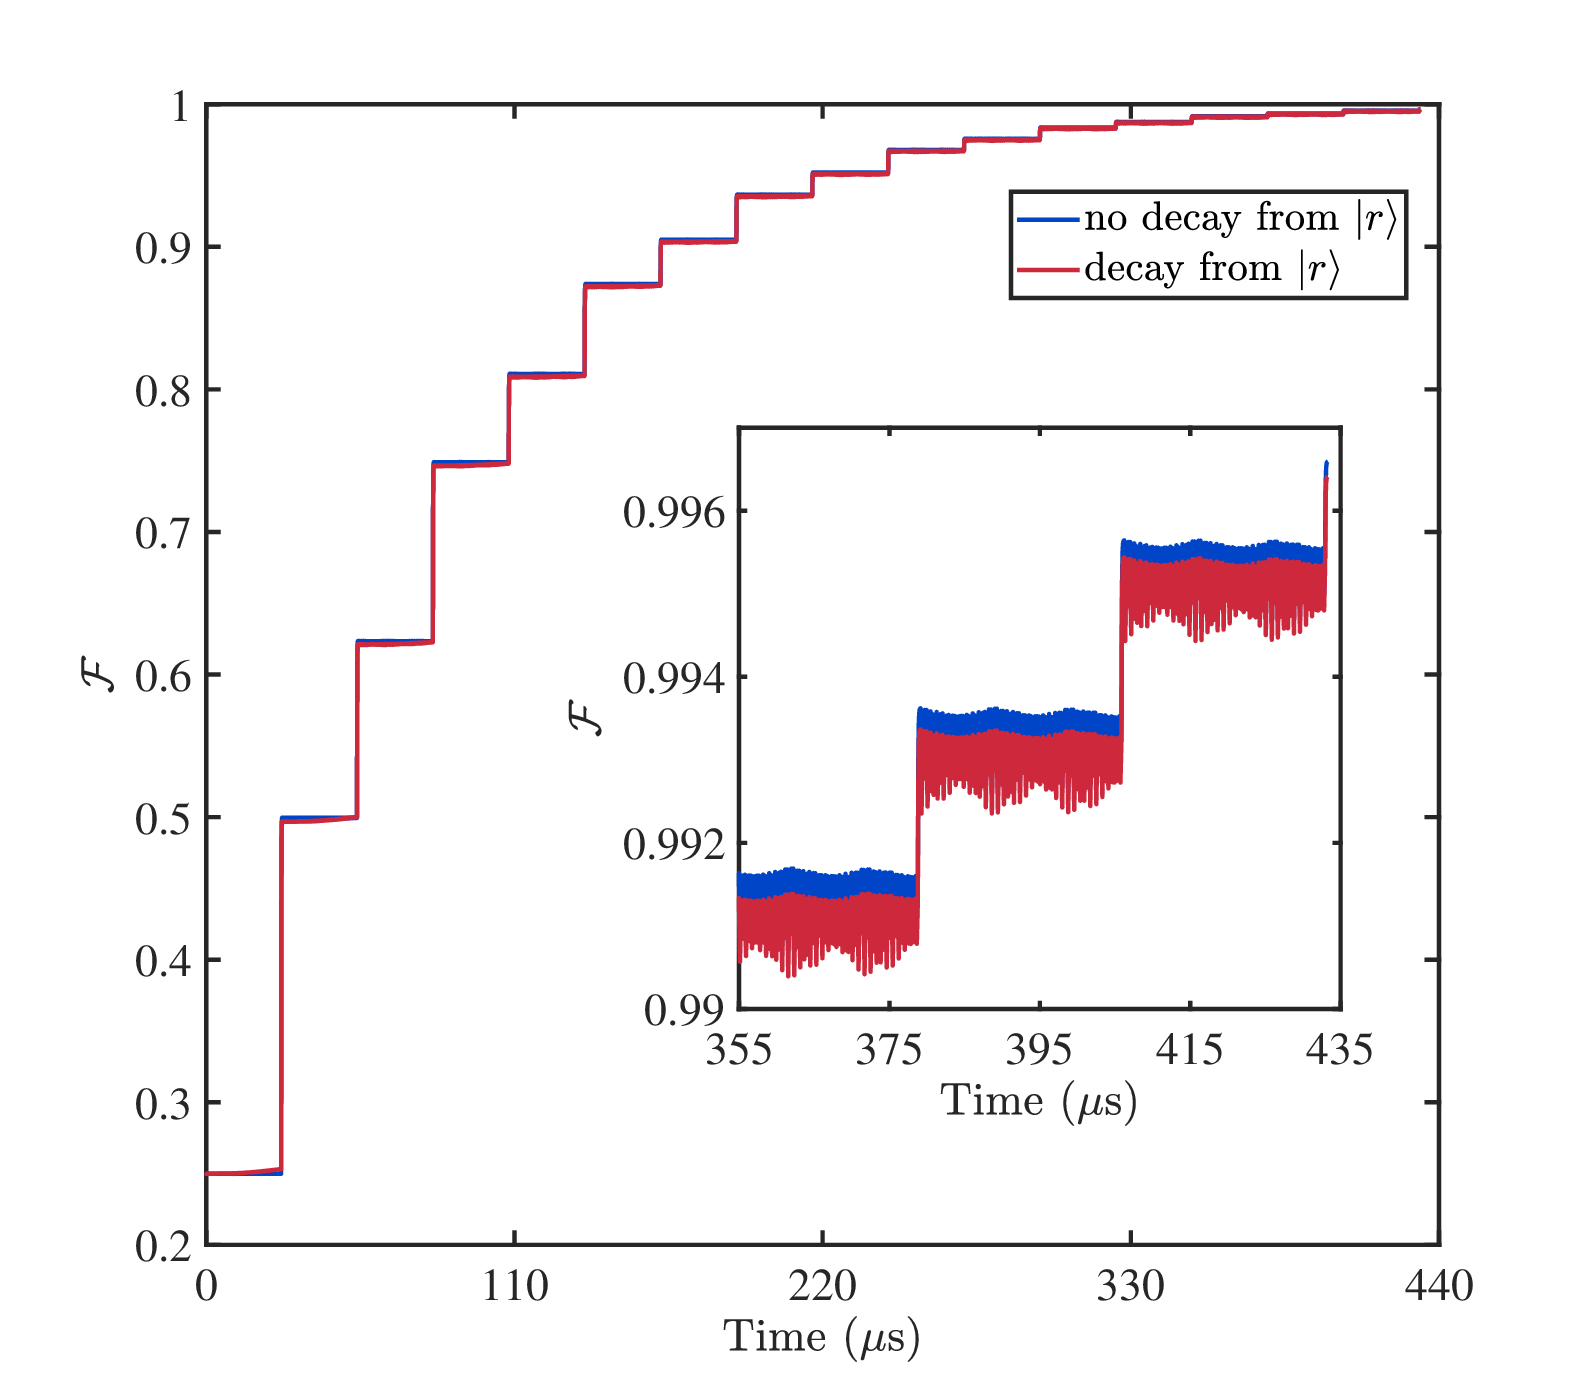}
	\caption{The comparison between the fidelity without and with decay from Rydberg state $|r\rangle$. The insert represents the amplification of the fidelity of the last interval. The decay rate is set as $\gamma_{r}/(2\pi) = 0.313$~kHz, and other parameters are the same as those in the main text.}\label{fig_VS_decay_r}
\end{figure}

\section{parallel stabilizer pumping for Accelerated generation of multipartite cluster states}

Reference~\cite{Bluvstein2022A} has achieved the preparation of multipartite 1D cluster states through a carefully crafted CZ gate scheme in experiments. 
By leveraging the mobility of atoms manipulated via optical tweezers, this approach enables cluster state generation in the minimal number of steps, albeit with a modest reduction in fidelity. This method can be seamlessly integrated into our framework to achieve the fastest possible cluster state preparation. Nevertheless, we propose an alternative approach with lower cost to accelerate the generation of multipartite cluster states through parallel stabilizer pumping.

Our proposed scheme divides the three-qubit bulk stabilizer operations into five sequential steps: (i)~$S_{2+5(n-1)}$, (ii)~$S_{3+5(n-1)}$, (iii)~$S_{4+5(n-1)}$, (iv)~$S_{5+5(n-1)}$, and (v)~$S_{6+5(n-1)}$, where $n = 1, 2, 3, \dots$. For the two-qubit boundary stabilizer operations, $S_1$ is incorporated into step (v), while $S_N$ is embedded in the step where the $S_{N-5}$ is located. As shown in Fig.~\ref{fig_pumping_order}, we display the operation order of the eight-qubit cluster state. To evaluate the acceleration performance, we conducted numerical simulations of six-, seven-, and eight-qubit cluster states, as shown in Fig.~\ref{accrelate_Cluster_678}. The six-qubit cluster state simulation employs the original Hamiltonian, while the seven- and eight-qubit cluster state simulations utilize the effective Hamiltonian. As the number of atoms increases, the acceleration effect becomes increasingly apparent.

\begin{figure}
	\centering
	\includegraphics[width=11.5cm]{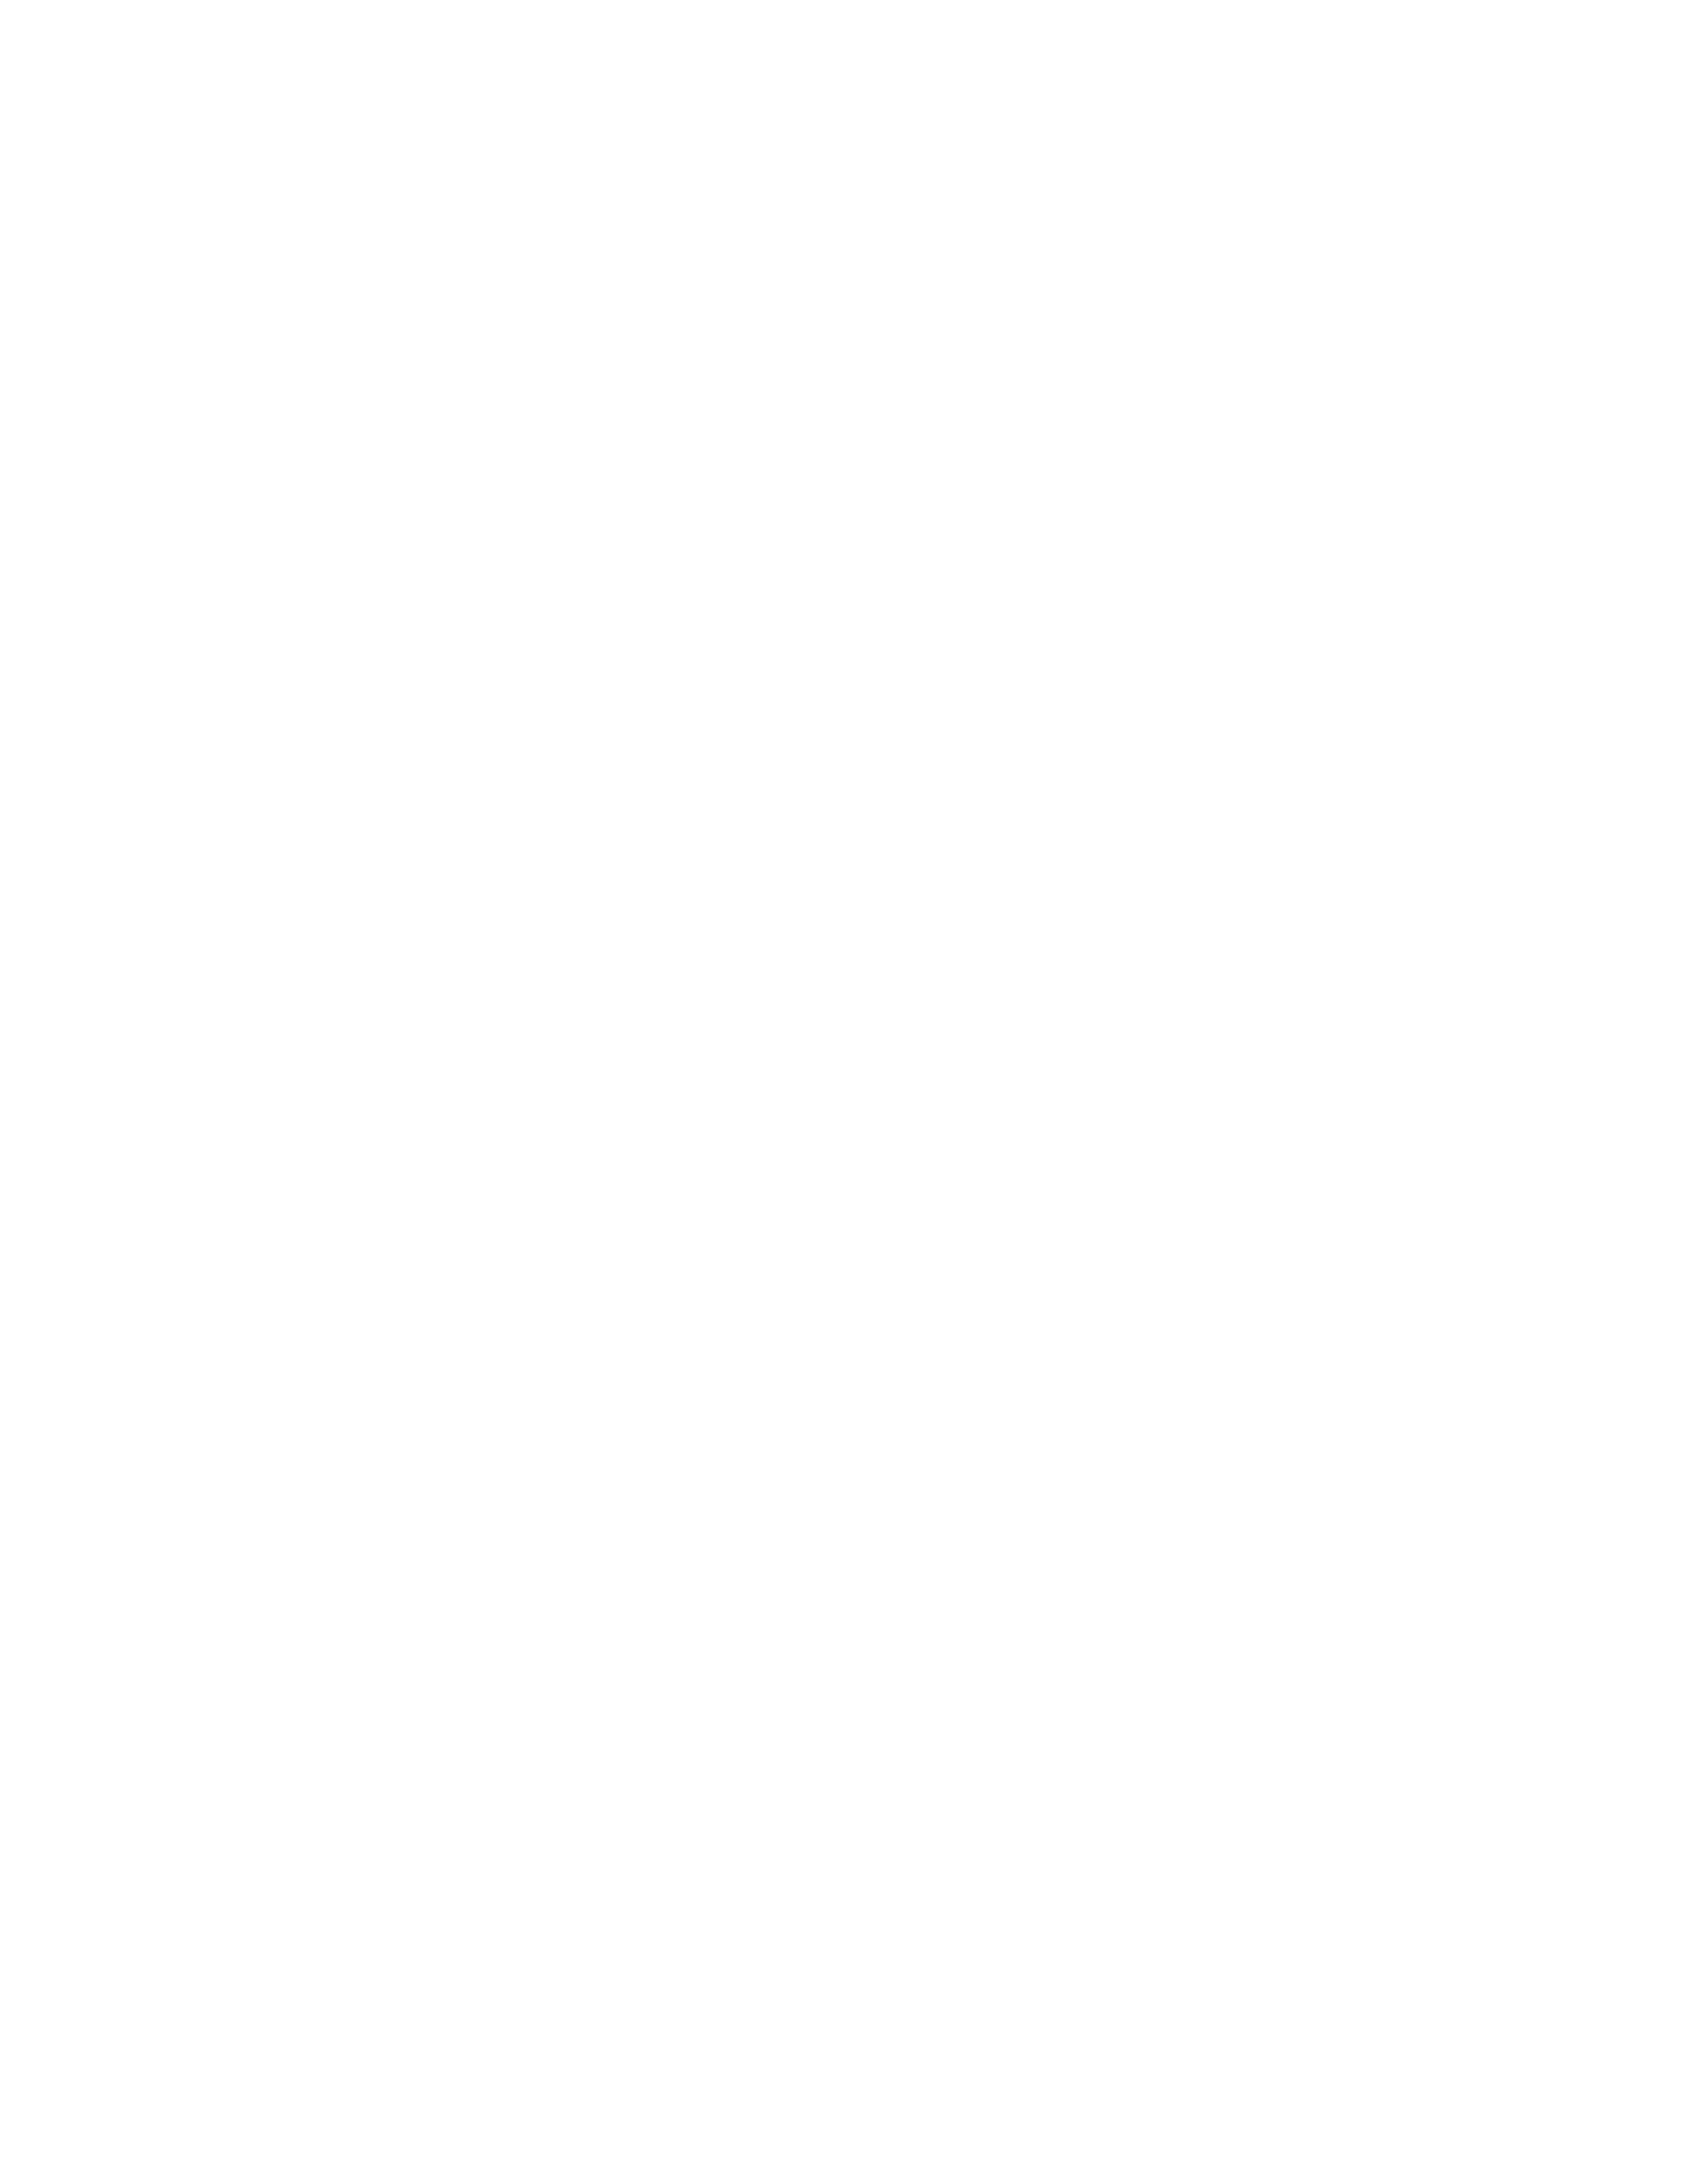}
	\caption{Schematic of the stabilizer operation sequence for an eight-qubit cluster state, executed as follows: (i)~$S_2$ and $S_7$, (ii)~$S_3$ and $S_8$, (iii)~$S_4$, (iv)~$S_5$, (v)~$S_1$ and $S_6$.}\label{fig_pumping_order}
\end{figure}
\begin{figure}
	\centering
	\includegraphics[width=17cm]{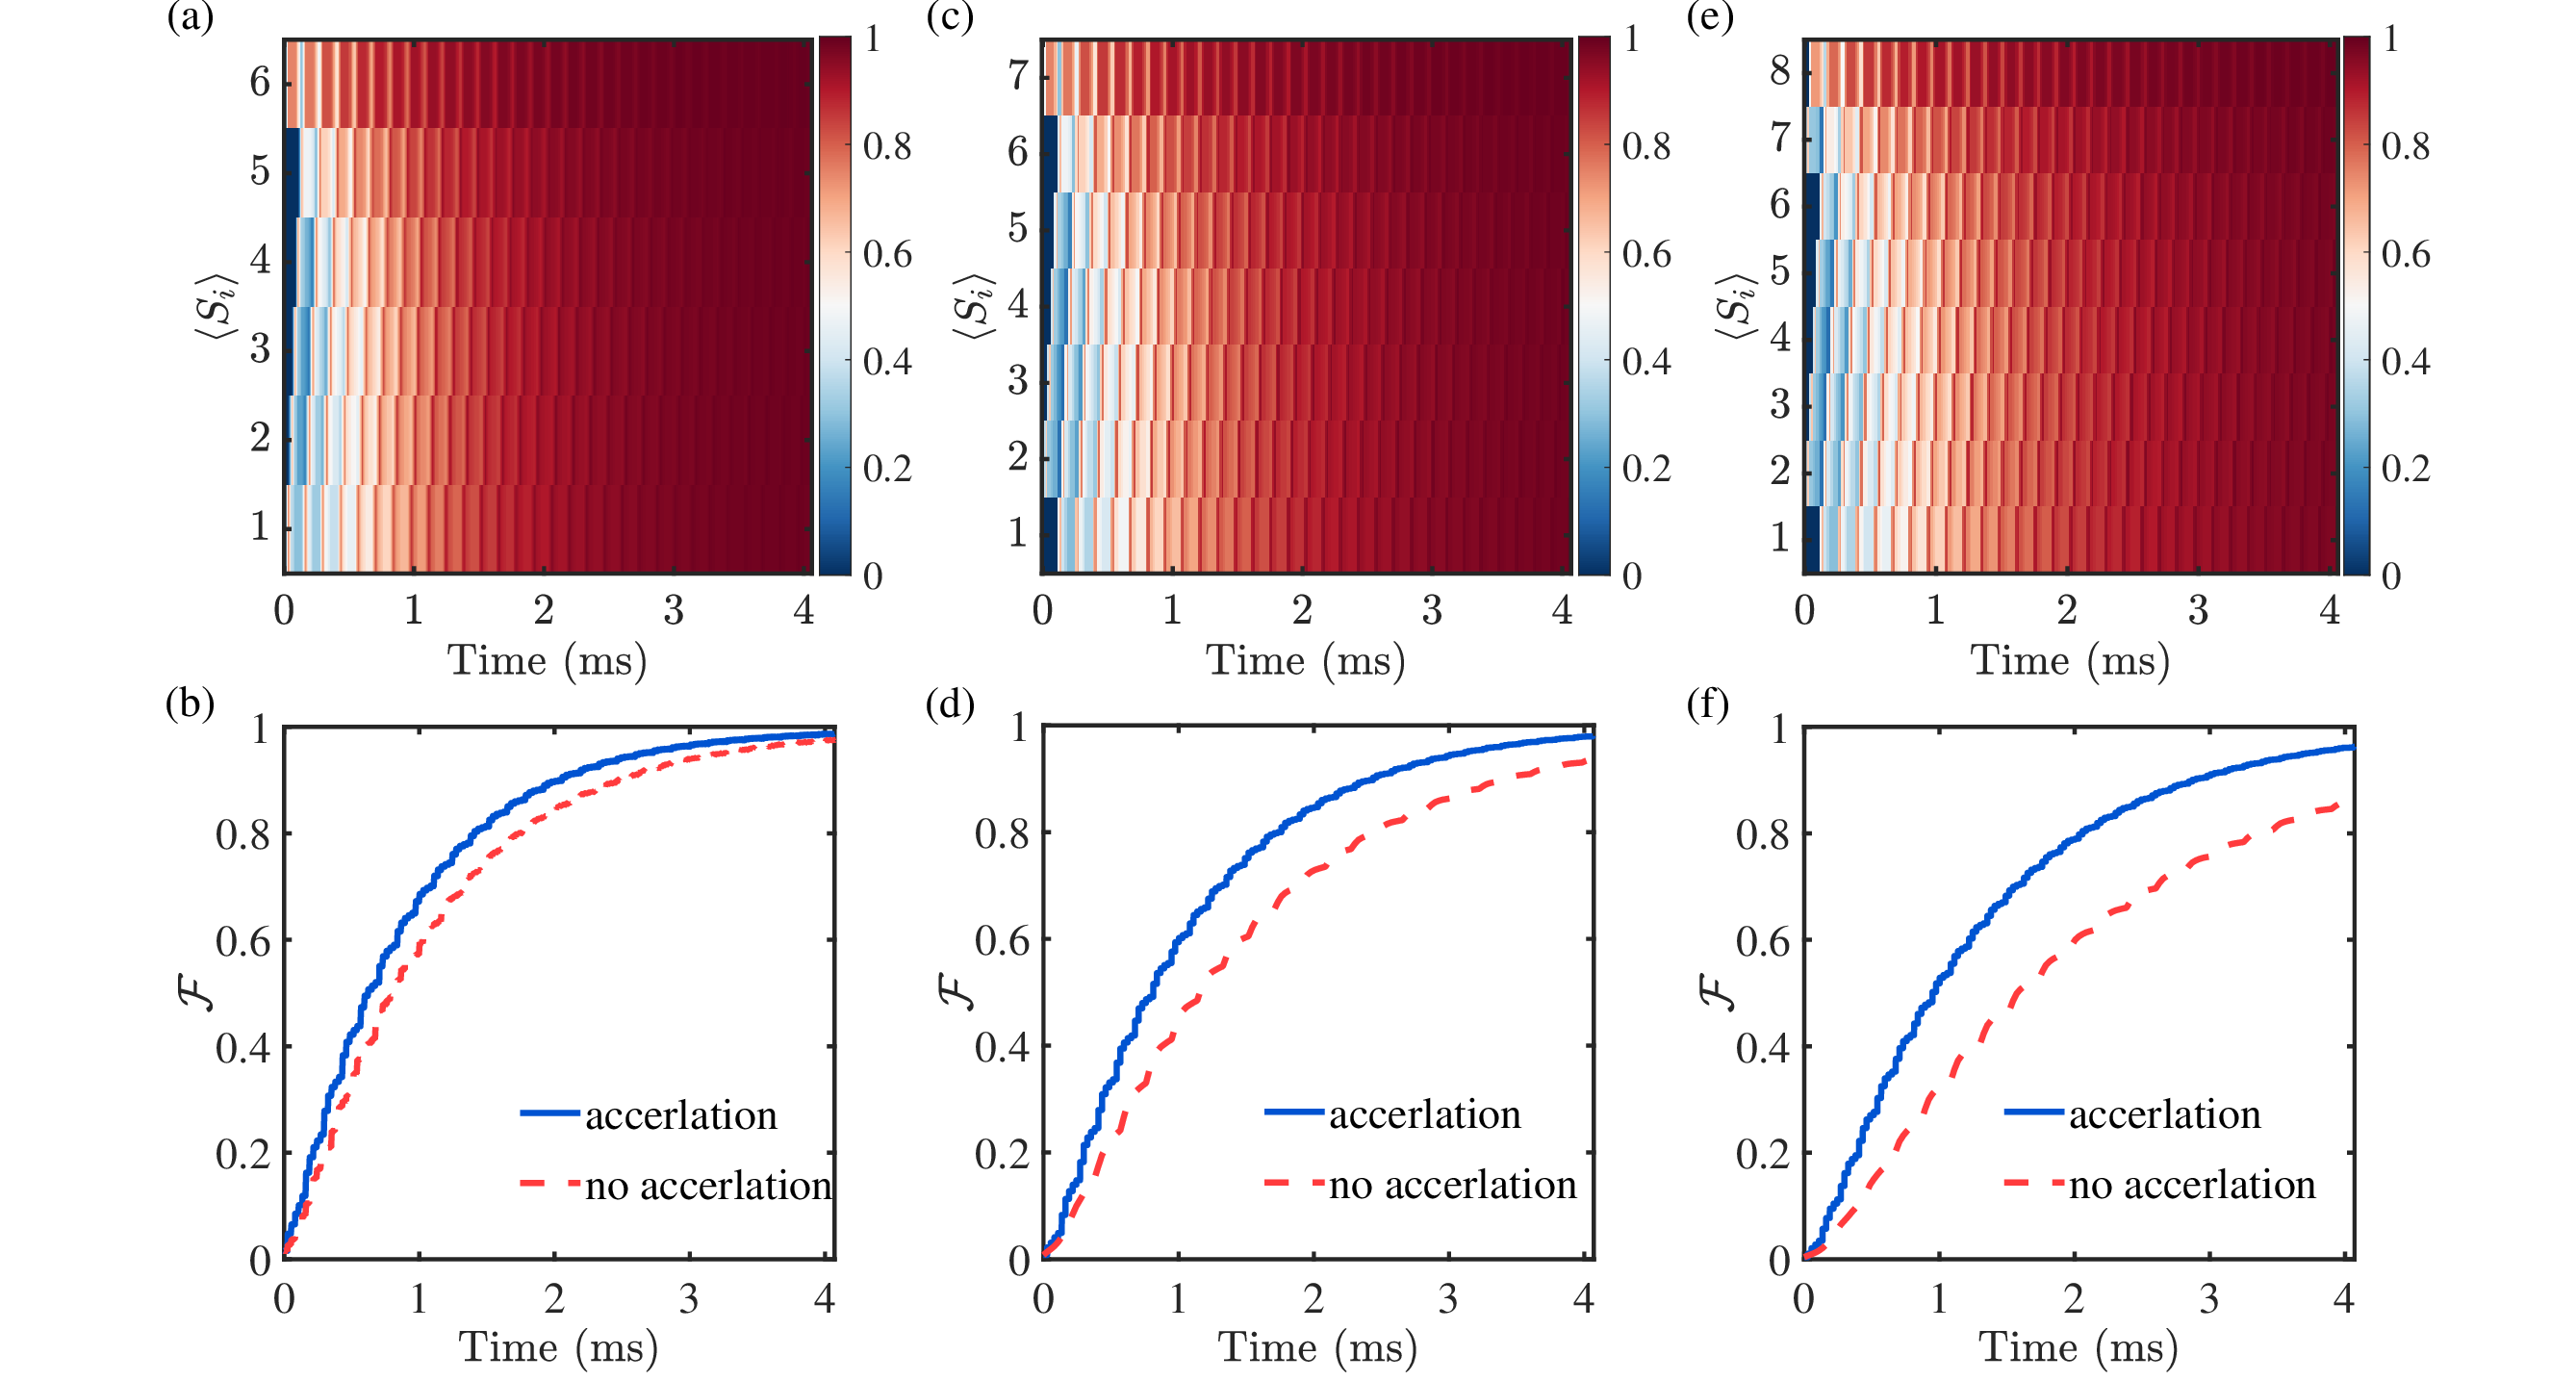}
	\caption{The acceleration of six- (a-b), seven- (c-d), and eight-qubit cluster state (e-f). (a), (c) and (e) display the temporal evolution of the expectation value of each stabilizer generator $\langle S_i\rangle$. (b), (d) and (f) display the comparison of fidelity with and without accelerations. The parameters are the same as that in the Figs.~4(a) and 4(b) of the main text.}\label{accrelate_Cluster_678}
\end{figure}

\section{The unique steady-state entanglement}\label{sec_steady}

In this section, we will discuss in detail the feasibility of a step-by-step pumping and dissipation scheme, in order to provide further extensions for this scheme.

\subsection{Uniqueness of the 1D $N$-qubit Cluster State govern by stabilizers generators $S$}

First, we provide a proof that a stabilizer group can stabilize the cluster states:
the stabilizer generators for an 1D $N$-qubit cluster state are given by the set $\mathcal{S}$:
\begin{equation}
    \mathcal{S} = \{ S_1=X_1 Z_2, \quad S_k=Z_{k-1}X_k Z_{k+1} \text{ for } k=2,\dots,N-1, \quad S_N=Z_{N-1}X_N \}.
\end{equation}

The $N$ stabilizer generators $S_i$ are mutually commuting and independent. They generate an Abelian group, known as the stabilizer group $\mathcal{G}$, which contains all possible products of the generators.
\begin{equation}
    \mathcal{G} = \left\{ \prod_{i \in K} S_i \mid K \subseteq \{1, \dots, N\} \right\}.
\end{equation}
%% 这个投影算符用幂等性和群重排定理可以证明。
This group has an order (number of elements) of $|\mathcal{G}| = 2^N$.

To find the common `+1' eigenspace (assume as the preparation target) of all these stabilizers, we can construct a projection operator $\Pi_{\text{stable}}$ by averaging all the elements of the group $\mathcal{G}$:
\begin{equation}
    \Pi_{\text{stable}} = \frac{1}{|\mathcal{G}|} \sum_{g \in \mathcal{G}} g = \frac{1}{2^N} \sum_{g \in \mathcal{G}} g.
\end{equation}
This operator projects any arbitrary state in the Hilbert space $\mathcal{H}$ (of dimension $2^N$) onto the stable subspace, which is the subspace of all states $|\psi\rangle$ satisfying $g|\psi\rangle = |\psi\rangle$ for all $g \in \mathcal{G}$.

The dimension of the stable subspace is equal to the rank of the projection operator, $\text{rank}(\Pi_{\text{stable}})$. For any projection operator, its rank is equal to its trace. Therefore, we can find the dimension of the subspace by calculating the trace of $\Pi_{\text{stable}}$:
\begin{equation}
    \text{rank}(\Pi_{\text{stable}}) = \text{Tr}(\Pi_{\text{stable}}) = \text{Tr}\left( \frac{1}{2^N} \sum_{g \in \mathcal{G}} g \right) = \frac{1}{2^N} \sum_{g \in \mathcal{G}} \text{Tr}(g).
\end{equation}

To evaluate this sum, we consider the trace of each element $g \in \mathcal{G}$. Each element is a Pauli string (a tensor product of Pauli matrices and the identity).

For the identity element $g = \mathcal{I}$, its trace is equal to the dimension of the Hilbert space:
\begin{equation}
    \text{Tr}(\mathcal{I}) = 2^N.
\end{equation}

For any other element $g \neq \mathcal{I}$, $g$ is a non-trivial Pauli string. The trace of any non-trivial Pauli matrix is zero, and thus the trace of any non-trivial Pauli string is also zero:
\begin{equation}
    \text{Tr}(g) = 0 \quad \text{for } g \neq \mathcal{I}.
\end{equation}

Substituting these results back into the expression for the rank, we find that all terms in the summation vanish except for the identity term:
\begin{equation}
    \text{rank}(\Pi_{\text{stable}}) = \frac{1}{2^N} \left[ \text{Tr}(\mathcal{I}) + \sum_{g \in \mathcal{G}, g \neq \mathcal{I}} \text{Tr}(g) \right] = \frac{1}{2^N} (2^N + 0) = 1.
\end{equation}

Since the rank of the projection operator $\Pi_{\text{stable}}$ is 1, the stable subspace is one dimensional. This proves that there exists a unique (up to a global phase) quantum state, the 1D $N$-qubit cluster state $|C_{N}\rangle$, that is simultaneously stabilized by all generators $S_i$.

\subsection{Analysis of the Realistic Pumping Scheme}

The proof above confirms a fundamental principle: the stabilizer set $\mathcal{S}$ mathematically defines a unique quantum state. It provides the theoretical justification for why the $N$-qubit cluster state $|C_N\rangle$ is the target steady state of the dissipation scheme based on stabilizers.

However, this elegant group-theoretic proof relies on an idealized assumption: the physical pumping process completely ``attacks" the entire negative eigenspace of every stabilizer generator. In a physical implementation related to experiments, this may not be the case. Defective attack on the negative eigenspace can break the perfect symmetry of the stabilizer group that underpins the projector formalism. Consequently, the systemic dynamics can no longer be described by the simple group projector $\Pi_{\text{stable}}$. As detailed in our main proposal, our scheme is designed such that the pumping of the bulk stabilizers' negative eigenstates is unavoidably incomplete. Specifically, for a stabilizer like $S_k = Z_{k-1}X_k Z_{k+1}$, the state $|1_{k-1} -_k 1_{k+1}\rangle$ is not directly excited. The previous proof, while correct for the ideal case, is not sufficient to guarantee the success of our realistic scheme. Therefore, we continue to provide a stronger and more general proof, which provides a fundamental theoretical explanation for the practical extension of further pumping and dissipation type schemes.

To rigorously analyze this more realistic scenario, we adopt a more fundamental and robust framework--system's kernel space, to directly model the physical pumping and dissipation scheme. This approach is more powerful because it only relies on the specific set of states $\{|j\rangle\}$ that are actually pumped by the lasers.

Define a total ``pump operator'' $\mathcal{P}$, which represents the sum of all ``pumping + dissipative'' channels in our scheme. It is constructed from the projectors onto all states $|j\rangle$ that are excited:
\begin{equation}
    \mathcal{P} = \sum_{j} P_j = \sum_{j} |j\rangle\langle j|.
\end{equation}
A quantum state $|\psi\rangle$ is a dark state (even a steady state) if and only if it is completely unaffected by the pumping. This means it must lie in the null space of the pump operator, denoted $\ker(\mathcal{P})$:
\begin{equation}
    \ker(\mathcal{P}) = \{ |\psi\rangle \in \mathcal{H} \mid \mathcal{P} |\psi\rangle = \mathbf{0} \}.
\end{equation}
Since all $P_j$ are positive semi-definite, this condition is equivalent to the requirement that $\langle j | \psi \rangle = 0$ for all pumped states $|j\rangle$.

The existence of a unique steady state is therefore guaranteed if and only if the dimension of this kernel is one:
\begin{equation}
    \dim[\ker(\mathcal{P})] = 1.
\end{equation}

We now apply this formalism to some practical schemes. The central issue can be expressed as: even with this reduced set of directly pumped states, is the dimension of the resulting kernel still one?

By applying the Rank-Nullity Theorem, the dimension of the kernel can be given by
\begin{equation}
    \dim[\ker(\mathcal{P})] = \dim(\mathcal{H}) - \text{rank}(\mathcal{P}).
\end{equation}
The rank of $\mathcal{P}$ is the number of linearly independent vectors in the set of pumped states $\{|j\rangle\}$.
%% This is precisely what is calculated by constructing the matrix $\mathcal{O}$ (whose rows are $\langle j|$) and finding its rank.

As rigorously analyzed in the main text, even with the exclusion of the $|1-1\rangle$-type states, the set of pumped states is sufficiently rich to ensure that it contains $2^N - 1$ linearly independent vectors. Consequently, the rank of the pump operator is $\text{rank}(\mathcal{P}) = 2^N - 1$. Therefore,
\begin{equation}
    \dim[\ker(\mathcal{P})] = 2^N - (2^N - 1) = 1.
\end{equation}
This proves that despite the incomplete direct pumping, our scheme still prepares a unique steady state. Finally, since we know by construction that the target cluster state $|C_N\rangle$ is orthogonal to all pumped states (as it is a +1 eigenstate of all stabilizers), it must be an element of the kernel. Since the kernel is one dimensional, it must be this unique steady state. We can thus state our final conclusion with mathematical precision:
\begin{equation}
    \ker(\mathcal{P}) = \text{span}\{|C_N\rangle\}.
\end{equation}

%%%%%%%%%%%%%%%%%%%%%%%

\subsection{The Pump Operator as a Constraint System: Uniqueness, Robustness, and Speed}

The dissipative preparation of a target state can be viewed as the application of a set of constraints on the system's Hilbert space. The pump operator, $\mathcal{P} = \sum_{j} \ket{j}\bra{j}$, defines this set, and a state $\ket{\psi}$ survives as a steady dark state only if it is orthogonal to all pumped states, i.e., $\braket{j|\psi}=0$ for all $\ket{j}$. The success of a preparation scheme therefore depends critically on whether the implemented constraints are sufficient to uniquely define the target state, and the nature of these constraints dictates the preparation speed.

\textbf{The Necessity of a Sufficient Constraint Set.} 
An insufficient set of constraints will fail to produce a unique steady state. If the subspace spanned by the pumped states is too small, the kernel of the pump operator will have a dimension greater than one, allowing for multiple, unwanted dark states. A clear example of this failure is found in a naive attempt to prepare a two-qubit cluster state, stabilized by $S_1=X_1Z_2$ and $S_2=Z_1X_2$. If one implements an incomplete pumping scheme that only imposes two constraints---for instance, by only pumping the states $\ket{-0}$ and $\ket{0-}$---the dark state subspace is two dimensional, that one is $C_2$ and the other is $1/\sqrt{3}(C_{2}^{+-} + C_{2}^{-+} + C_{2}^{--})$ composed of three other orthogonal states. This scheme fails because the constraints are inadequate to eliminate all states orthogonal to the target Bell state.

\textbf{Robustness via Indirect and Overlapping Constraints.}
Our realistic scheme for preparing the cluster state avoids this failure, even though it employs an incomplete set of direct constraints. The key to its success lies in the power of indirect, overlapping constraints. A ``constraint" is fundamentally a mathematical condition of non-orthogonality: any pumped state $\ket{j}$ constrains any state $\ket{\psi}$ as long as their inner product $\braket{j|\psi}$ is non-zero. For instance, in the three-qubit scheme, we do not directly pump the state $\ket{1_1-_21_3}$. However, this state is still constrained by the implemented pumping, such as the projectors $\ket{-_{1}0_{2}}\bra{-_{1}0_{2}}\otimes \mathcal{I}_{3}$ and $ \mathcal{I}_{1} \otimes \ket{0_{2}-_{3}}\bra{0_{2}-_{3}}$, which have non-zero overlaps with $\ket{1_1-_21_3}$. This non-zero inner product constitutes a valid, albeit indirect, constraint that prevents $\ket{1_1-_21_3}$ from being a dark state. The robustness of our scheme stems from the fact that the full set of these indirect constraints is sufficient to compensate for the missing direct ones, ensuring a unique steady state.

\textbf{Reduced Dissipative Channels and Preparation Speed.}
Finally, while these overlapping constraints guarantee uniqueness, the reduction in the total number of decay channels adversely affects the preparation speed. This performance degradation can be explained by analyzing the systemic gap of the Floquet Liouvillian $\mathcal{L}_F(t)$, given by $g_{F} = \min_{\lambda'_k \neq 0} |\text{Re}(\lambda'_k)|$, where $\lambda'_k(t)$ are the eigenvalues of $\mathcal{L}_F(t)$. Each dissipative channel corresponding to the pumping of a specific state $\ket{j}$ contributes a loss term to the Floquet Liouvillian. In an ideal case where all negative eigenstates of all stabilizers are pumped, the Floquet Liouvillian $\mathcal{L}_{F_{\text{ideal}}}(t)$ possesses a certain gap $g_{F_{\text{ideal}}}$. In our realistic scheme, the failure to excite some states (such as $\ket{1_{k-1}-_k 1_{k+1}}$) means that our Floquet Liouvillian $\mathcal{L}_{F_{\text{real}}}(t)$ is missing these corresponding dissipative terms. The removal of these direct decay pathways can be shown to reduce the overall magnitude of dissipation, leading to a smaller dissipative gap, i.e., $g_{F_{\text{real}}} \le g_{F_{\text{ideal}}}$. Intuitively, quantum state populations that could have rapidly decayed through a missing direct channel must now follow more complex, multi-step paths to be dissipated by the remaining channels. These slower, indirect pathways are associated with eigenvalues closer to zero, thus shrinking the gap. 

A prime example is the stabilizer pumping of three-qubit cluster state. According to stabilizer $Z_{1}X_{2}Z_{3}$, we consider four cases of stabilizer pumping, including one pump state ($|0-0\rangle$), two pump states ($|1+0\rangle, |0-0\rangle$), three pump states ($|0+1\rangle, |1+0\rangle, |0-0\rangle$), and four pump states ($|0+1\rangle, |1+0\rangle, |0-0\rangle, |1-1\rangle$). The quasi energies of Floquet Liouvillian is shown in Fig.~\ref{Cluster3_LF_QES}, which all have same and unique zero-energy state $|r_{0}\rangle\rangle = |C_{3}\rangle \otimes |C_{3}\rangle$ satisfying $\mathcal{L_{F}}|r_{0}\rangle\rangle = 0$. They (one-, two-, and three-pump case), lacking its direct decay channel via the $S_2$ pump, is instead targeted by the pumps for the adjacent stabilizers $S_1=X_1Z_2$ and $S_3=Z_2X_3$. This forces its population into a slower, multi-step decay process, ultimately shrinking the dissipative gap. Consequently, the preparation time, which scales as $T_{\text{prep}} \sim 1/g_{F}$, is prolonged. Figure~\ref{Cluster3_LF_QES} displays that gap decreases with the reduction of pump terms. This analysis confirms that while our scheme is robust in achieving the target state, it comes at the cost of reduced preparation efficiency.

\begin{figure}
	\centering
	\includegraphics[width=18cm]{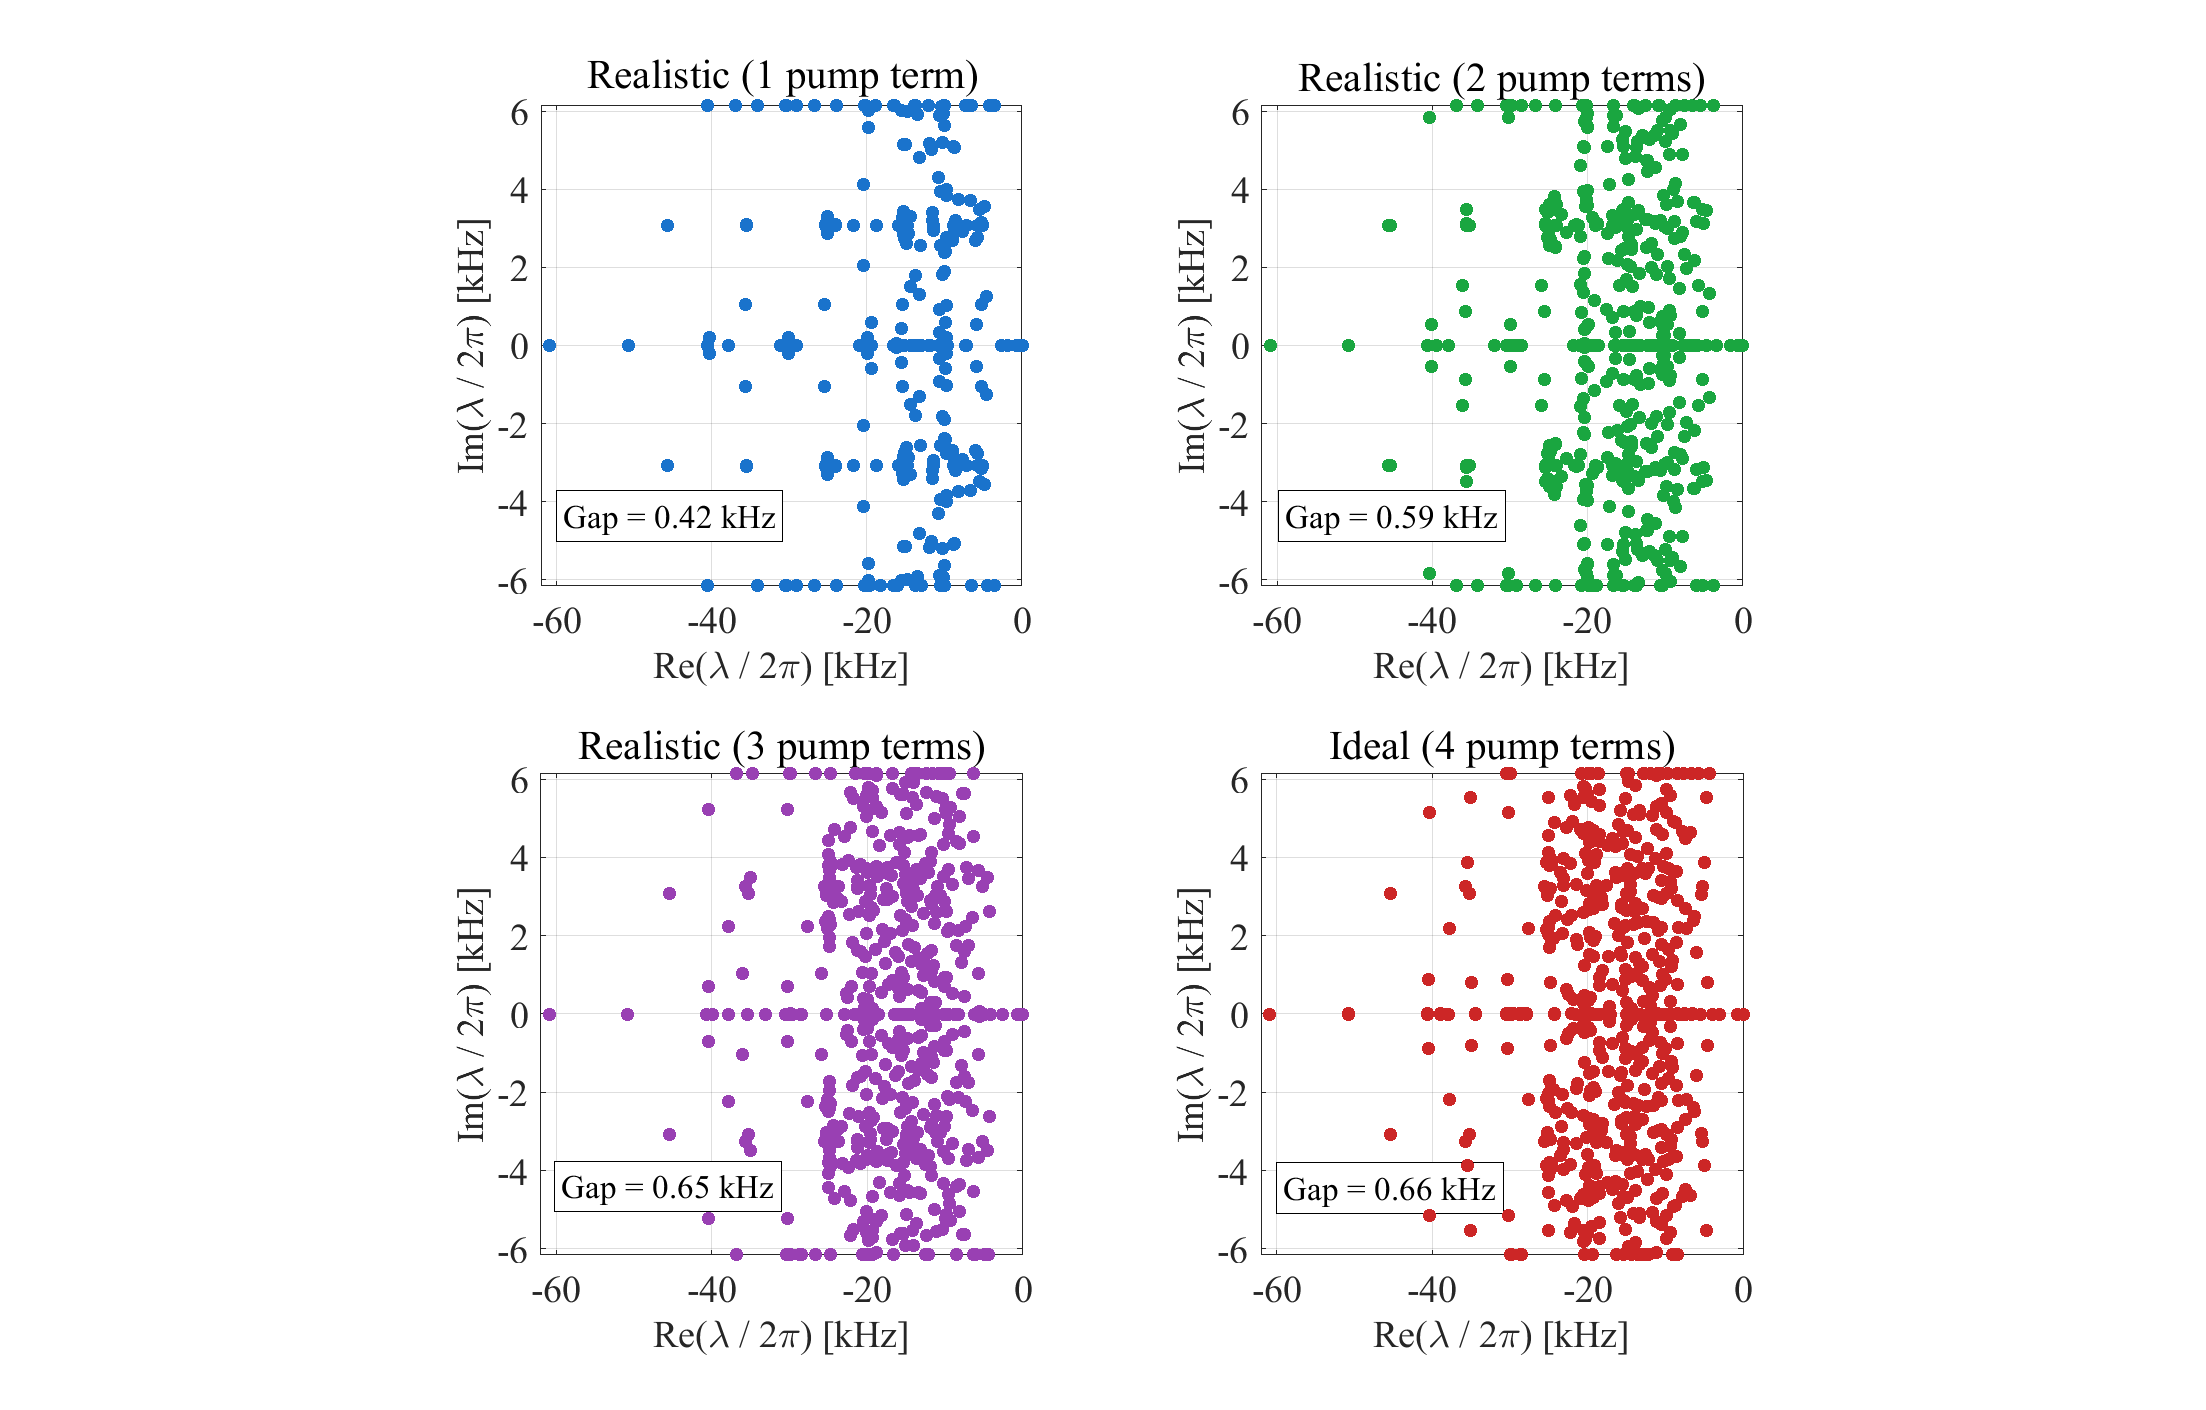}
	\caption{Quasienergy of Floquet Liouvillian achieving three-qubit cluster state. According to the pumping of stabilizer $Z_{1}X_{2}Z_{3}$, it is divided into four situations: one pump state ($|0-0\rangle$), two pump states ($|1+0\rangle, |0-0\rangle$), three pump states ($|0+1\rangle, |1+0\rangle, |0-0\rangle$), and four pump states ($|0+1\rangle, |1+0\rangle, |0-0\rangle, |1-1\rangle$). These one, two, and three pump terms correspond to possible physical reality, while four pump terms correspond to the ideal state. Here the stabilizer pumping in Floquet Hamiltonian has been used by effective Hamiltonian derived by the way in section.~\ref{sec:eff_Ham}. The parameters in effective scheme are set as $\mathcal{N}=100$, $\Omega= 2\pi\times 5$~MHz, $\alpha=0.6$, $\Omega t_1 = \pi/\mathcal{N}$, and $\int_{0}^{t_{2}}\Omega_{b}(t)dt = \pi$.}\label{Cluster3_LF_QES}
\end{figure}

%%%%%%%%%%%%%%%%%%%%%%%

\section{Extension of pumping and dissipation scheme based on stabilizers}

Based on the theoretical proof in the previous chapter, we further expand our approach in this chapter.

\subsection{One-dimensional based-complete-stabilizers stationary dynamics}

We first point out that dynamics based on complete stabilizer operations can also be achieved. For the bulk stabilizers $S_{k} = Z_{k-1}X_{k}Z_{k+1}$, we can use two times excitation and dissipation to achieve it. 

(i) Illuminate atoms with lasers to achieve an effective Hamiltonian described as 
\begin{equation}
    H_{S_{k}}^{(i)} = \frac{\Omega_\text{eff}}{2}(|r_{k-1}+_{k}0_{k+1}\rangle\langle 1_{k-1}+_{k}0_{k+1}| + |0_{k-1}r_{k}0_{k+1}\rangle\langle 0_{k-1}-_{k}0_{k+1}| + |0_{k-1}+_{k}r_{k+1}\rangle\langle 0_{k-1}+_{k}1_{k+1}|) + {\rm H.c.},
\end{equation}
with driven interval $T_{(i)} = \pi/\Omega_{\text{eff}}$.

(ii) Illuminate atoms with lasers to achieve an effective Hamiltonian described as 
\begin{equation}
    H_{S_{k}}^{(ii)} = \frac{\Omega_\text{eff}}{2}(|1_{k-1}r_{k}1_{k+1}\rangle\langle 1_{k-1}-_{k}1_{k+1}|) + {\rm H.c.},
\end{equation}
with the same driven interval $T_{(ii)} = \pi/\Omega_{\text{eff}}$. After completing these two steps, our operation sequence conforms to the driving principle based on the perfect bulk stabilizers $S_{k}$.

The remaining task is to provide the implementation method for effective Hamiltonian $H_{S_{k}}^{(ii)}$. We can execute these two Hamiltonians 
\begin{eqnarray}
    H_{a_{(ii)}}^{S_{k}}(t) &=& \frac{\Omega_{a}}{2}(\mathcal{I}_{k-1}\otimes|r_{k}\rangle\langle -_{k}|\otimes\mathcal{I}_{k+1}) + {\rm H.c.} + H_{V},\cr\cr
    H_{b_{(ii)}}^{S_{k}}(t) &=& \frac{\Omega_{b}(t)}{2}\cos(\Delta t)(|r_{k-1}\rangle\langle 0_{k-1}|\otimes\mathcal{I}_{k}\otimes\mathcal{I}_{k+1} + \mathcal{I}_{k-1}\otimes\mathcal{I}_{k}\otimes|r_{k+1}\rangle\langle 0_{k+1}|) + {\rm H.c.} + H_{V}.\nonumber
\end{eqnarray}
At this point, we can achieve stationary entanglement generation in an ideal way.

\subsection{Implementation of two-dimensional cluster state}

In the main text we have considered the implementation of 1D cluster state and the elementary CNOT gate, which meet the basic requirements of one-way quantum computing. Now, we further propose the implementation of two-dimensional (2D) cluster state combining the previously promoted theories. As shown in Figs.~\ref{fig:2D_lattice}(a) and~\ref{fig:2D_lattice}(b), we separately propose 2D cluster state with structures of triangular lattice and square lattice. Taking the six-qubit cluster states with stabilizer generators $\{X_{1}Z_{2}, Z_{1}X_{2}Z_{3}Z_{5}, Z_{2}X_{3}, X_{4}Z_{5}, Z_{2}Z_{4}X_{5}Z_{6}, Z_{5}X_{6}\}$ in two structures as an example, we demonstrate the implementation methods.

In fact, 2D six-qubit cluster state only requires two- and four-qubit stabilizer pumping, such that two kinds of structures have the same operations, in which we need to consider the excitation sum of at least three terms for two four-qubit stabilizer pumping to successfully implement our scheme (The pump operator has complete constraints). For example, this can be selected as
\begin{eqnarray}
    H_2^{f_{1}} = \frac{\Omega}{2}|0_{1}r_{2}0_{3}0_{5}\rangle\langle 0_{1}-_{2}0_{3}0_{5}|+\text{H.c.},\cr\cr
    H_2^{f_{2}} = \frac{\Omega}{2}|1_{1}r_{2}1_{3}1_{5}\rangle\langle 1_{1}+_{2}1_{3}1_{5}|+\text{H.c.},\cr\cr
    H_5^{f} = \frac{\Omega}{2}|0_{2}0_{4}r_{5}0_{6}\rangle\langle 0_{2}0_{4}-_{5}0_{6}|+\text{H.c.}
\label{eq:4_qubit_stabilizer}
\end{eqnarray}

As shown in Fig.~\ref{Cluster6_2D_effective}, the numerical simulation by the effective Hamiltonians displays the feasibility of the scheme.

 \begin{figure}
 	\centering
 	\includegraphics[width=15cm]{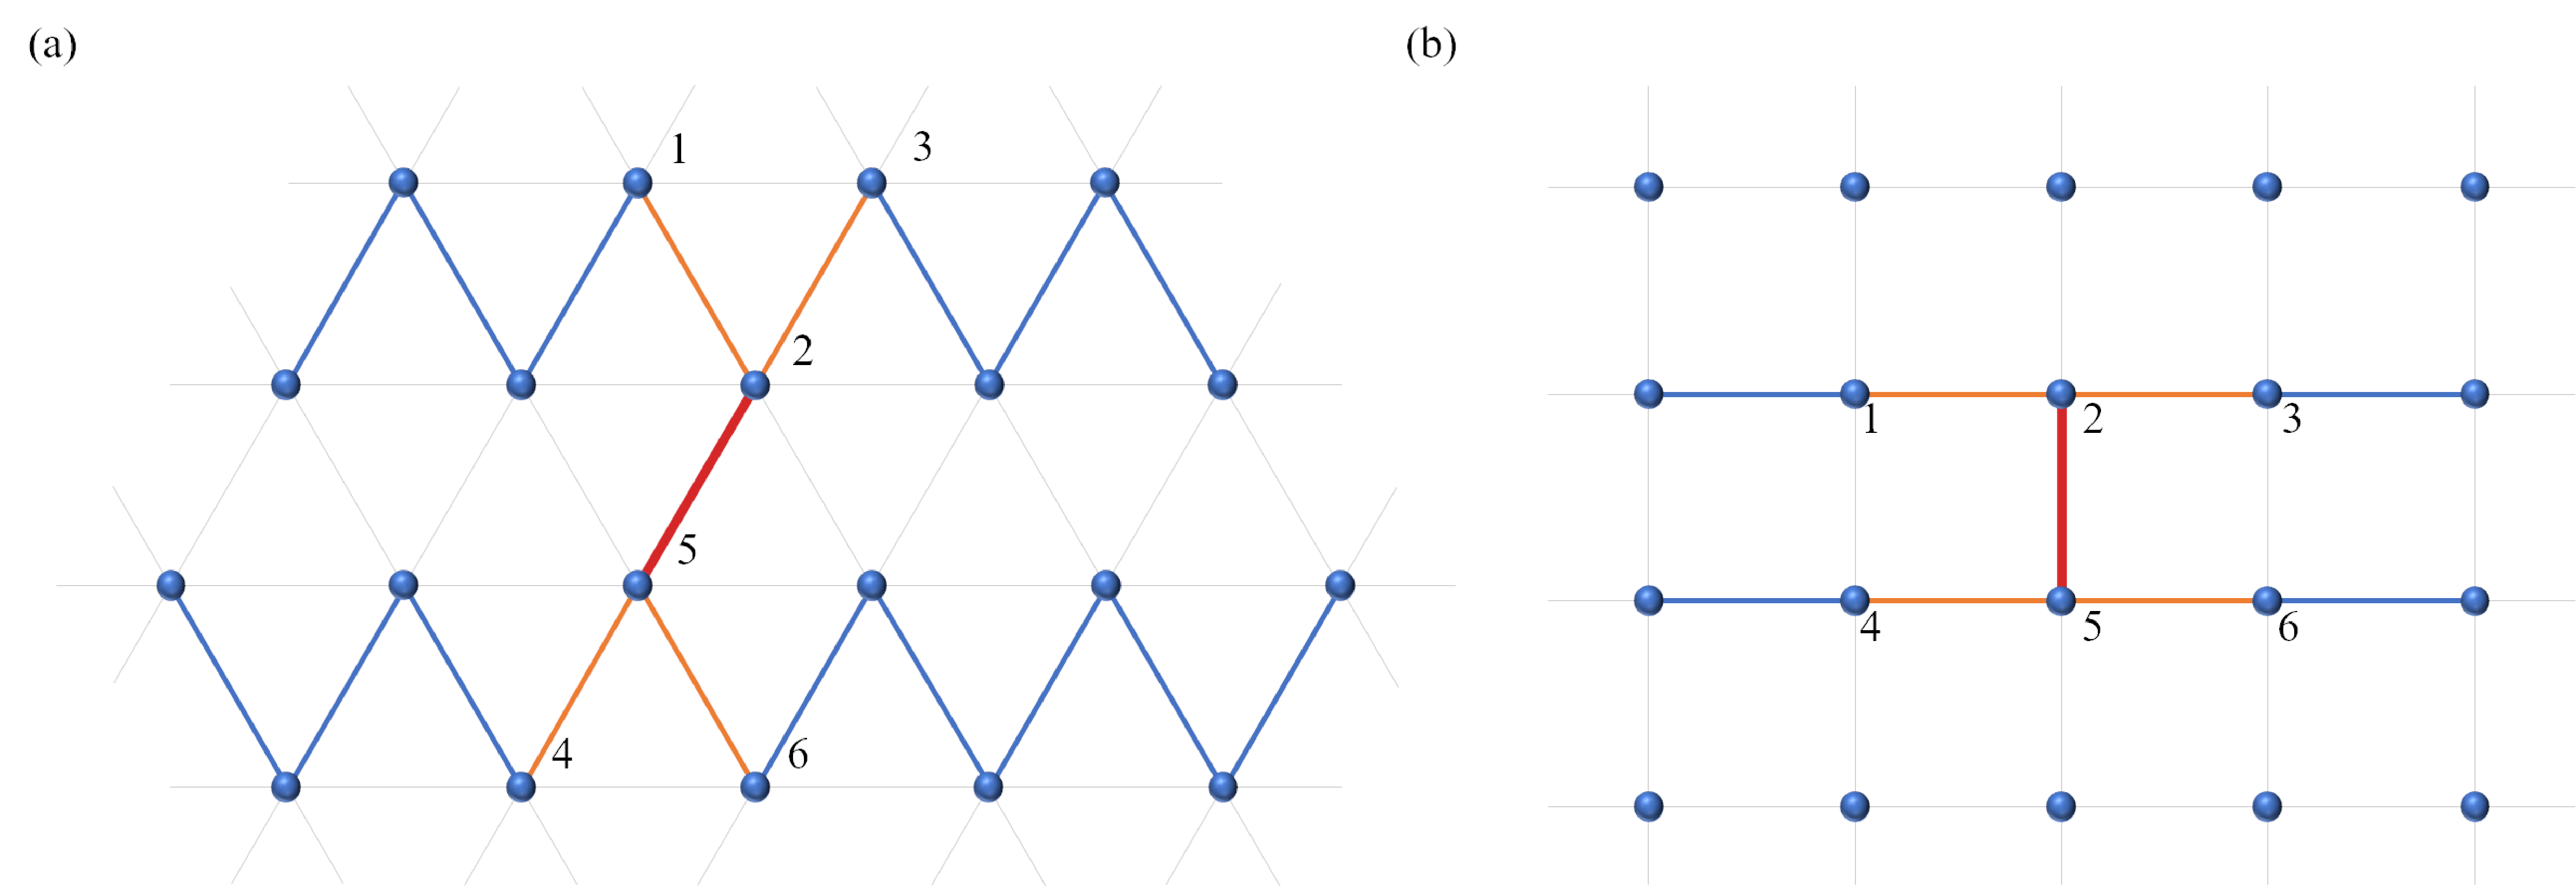}
 	\caption{Structures of 2D cluster states formed by triangular lattice (a) and square lattice (b), where the 1D cluster states are marked by blue lines, appearing jagged in structure (a) and straight in structure (b). The 2D six-qubit cluster states are marked by a yellow line, with the edges connecting two 1D three-qubit cluster states highlighted in red.}\label{fig:2D_lattice}
 \end{figure}

\begin{figure}
	\centering
	\includegraphics[width=8.2cm]{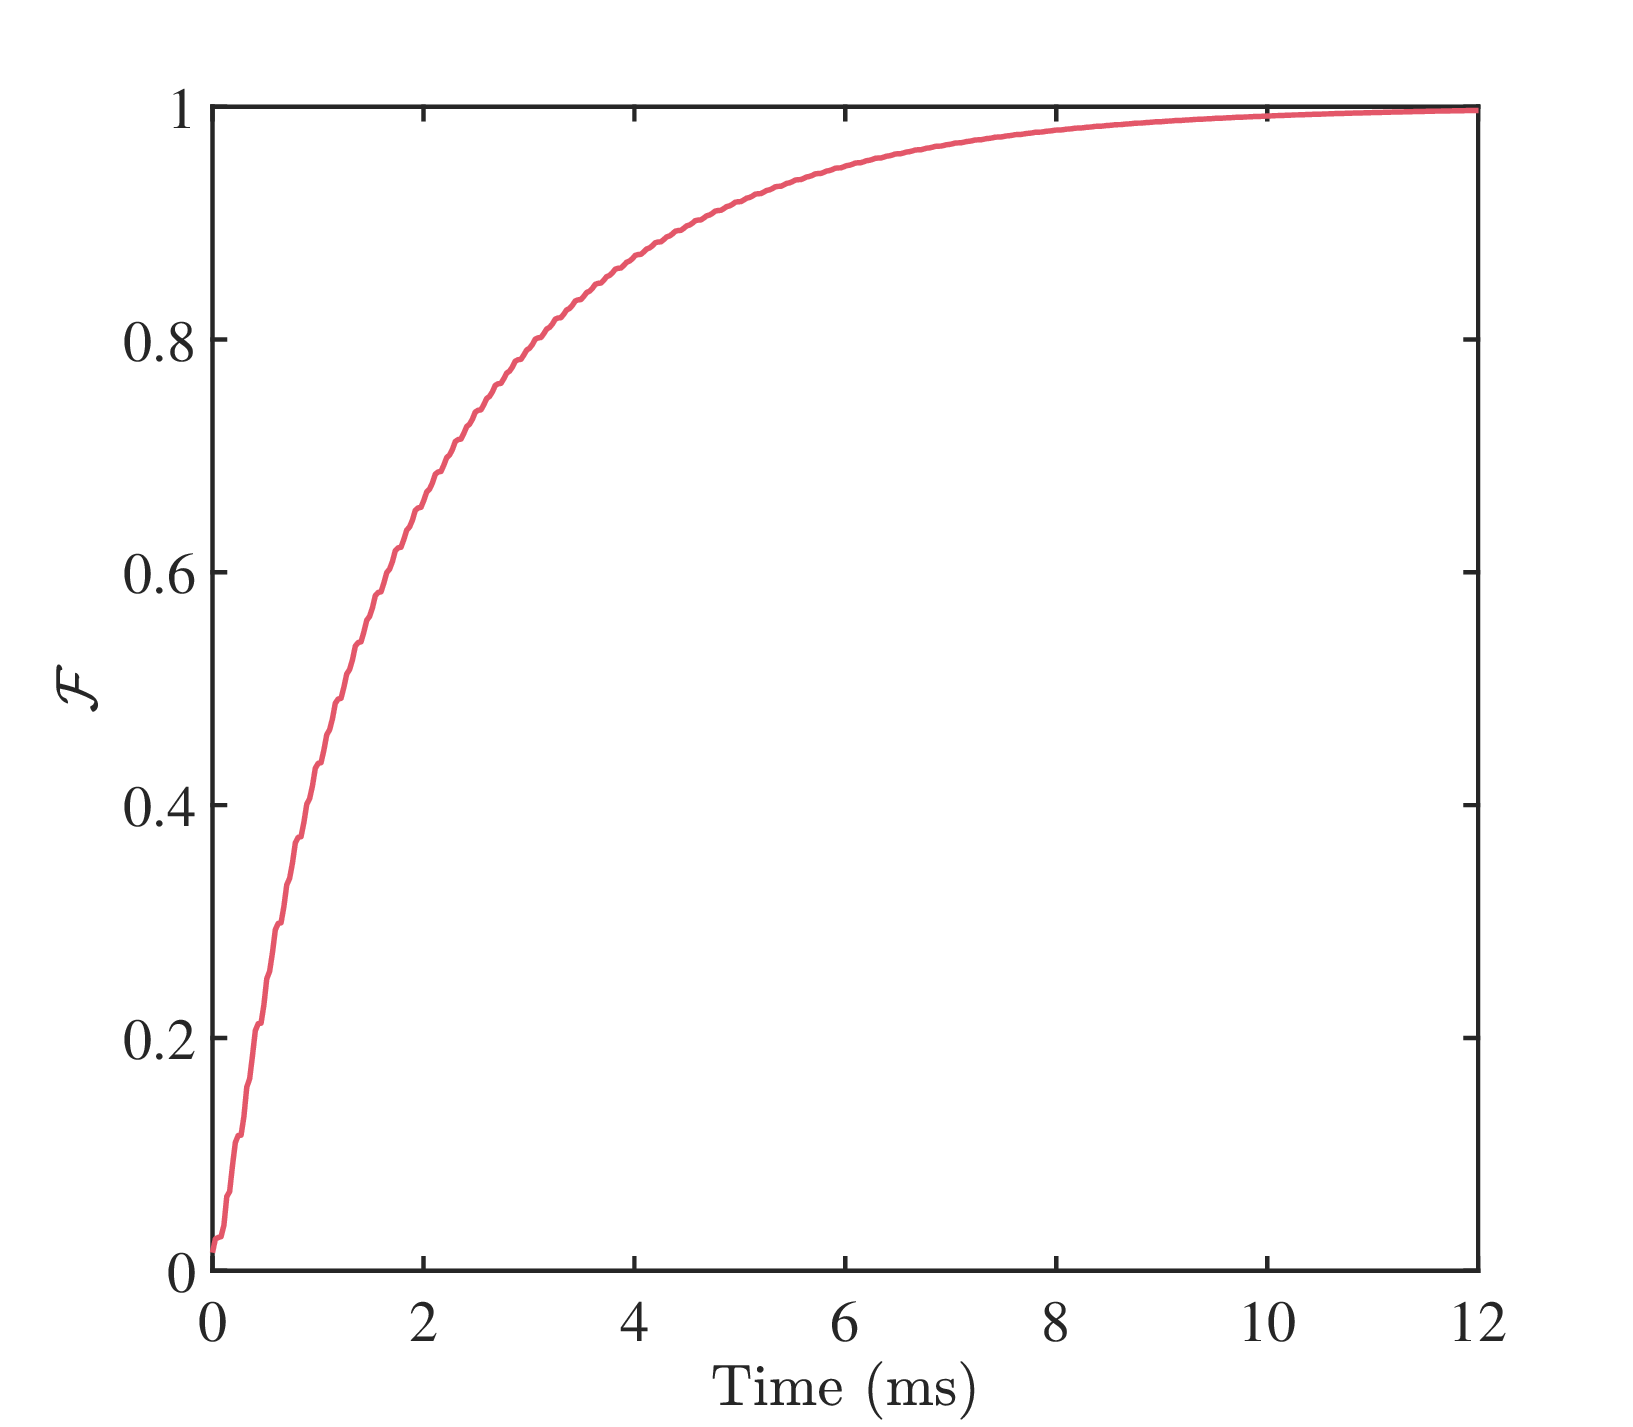}
	\caption{Preparation of 2D six-qubit cluster state by effective Hamiltonian structured in Fig.~\ref{fig:2D_lattice}. Under the consideration of effective excitation, both structures (a) and (b) in Fig.~\ref{fig:2D_lattice} can achieve perfect excitation of two-qubit stabilizers, while the same effective excitation Hamiltonians in Eq.~(\ref{eq:4_qubit_stabilizer}) are required for four-qubit stabilizers, thus they have the same effective evolution results. The parameters in effective scheme are set as $\Omega = 2\pi\times 5$~MHz, $\alpha = 0.6$, and $\mathcal{N}=100$.}\label{Cluster6_2D_effective}
\end{figure}

 \section{Purification of cluster states}

Here we make some additions to the purification scheme in the main text. Our approach facilitates the purification of cluster states, with the purification speed determined by the initial purity of the state. Define the initial impure three-qubit cluster state as
\begin{equation}
    |C_3^p\rangle = \cos(\beta) |+0+\rangle + \sin(\beta) |-1-\rangle.
\end{equation}
After \( \mathbb{N} \) cycles of the purification process, the pure three-qubit cluster state \( |C_3\rangle \) is obtained. To evaluate the performance, we numerically simulate the fidelity \( \mathcal{F} = \text{Tr}[\rho(t) \rho_{C_3}] \) with $\rho_{C_3} = |C_3^p\rangle\langle C_3^p|$, and the purity \( P_C = \text{Tr}[\rho^2(t)] \), as shown in Fig.~\ref{GHZ_original_mixed_purify}. The contour line corresponding to a fidelity (or purity) of 0.99 illustrates the purification speed. The purification is fastest when \( \beta \) approaches \( \pi/4 \) or \( 5\pi/4 \), and slowest when \( \beta \) approaches \( 3\pi/4 \) or \( 7\pi/4 \).

 \begin{figure}
 	\centering
 	\includegraphics[width=15cm]{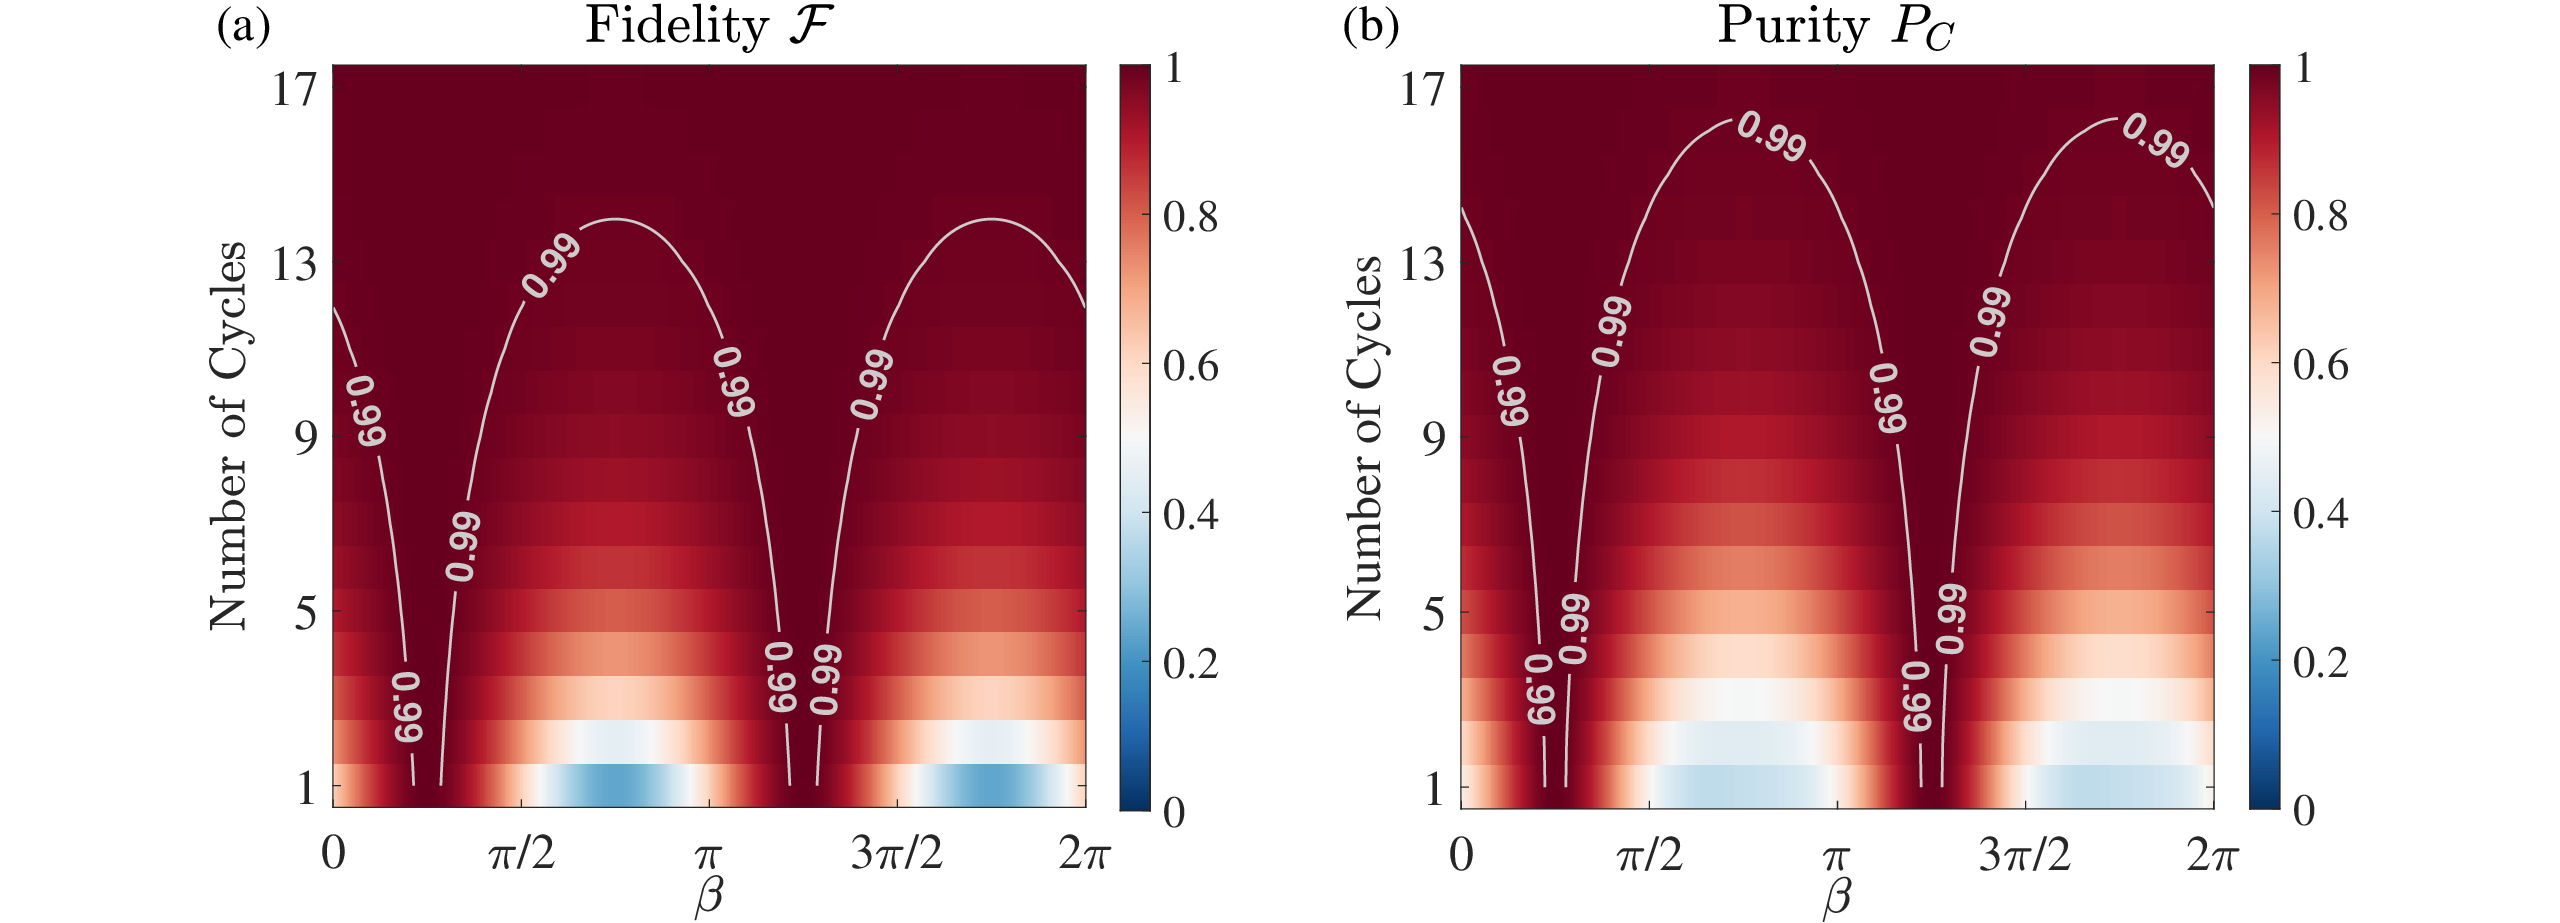}
 	\caption{Purification of the three-qubit cluster state \( |C_3\rangle \), initialized as \( |C_3^p\rangle \). (a) Fidelity as a function of the parameter \( \beta \) and the number of cycles \( \mathbb{N} \). (b) Purity as a function of \( \beta \) and \( \mathbb{N} \). Contour lines indicate a probability of 0.99. The parameters are the same as that in the Fig.~4(d) of the main text.}\label{GHZ_original_mixed_purify}
 \end{figure}

\section{Experimental proposal}

\begin{figure}
	\centering
	\includegraphics[width=1\linewidth]{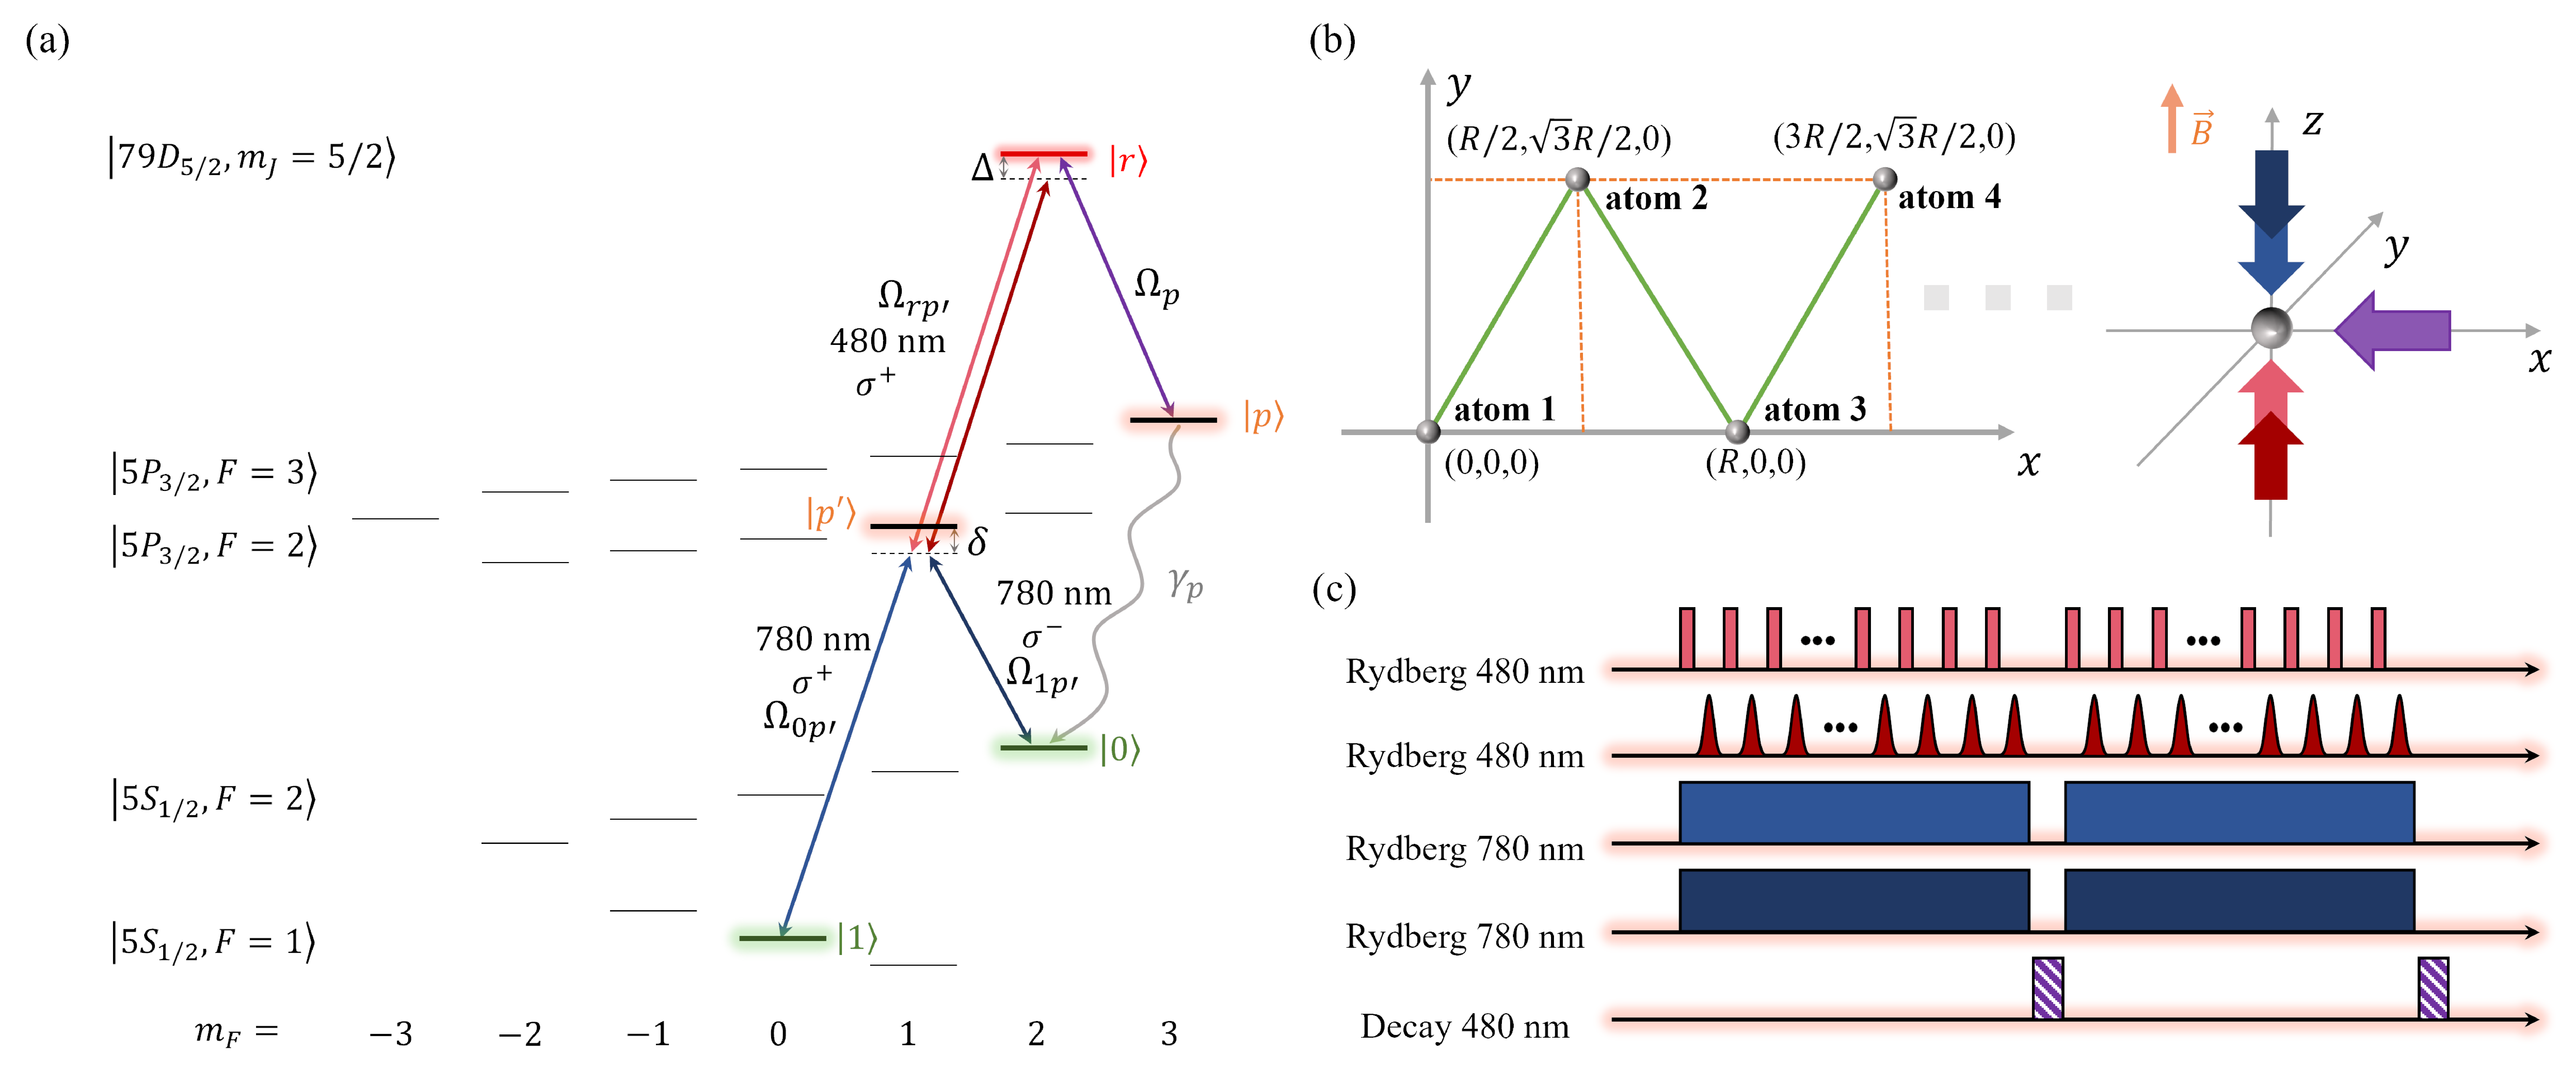}
	\caption{Schematic diagrams illustrating the experimental setup. (a) Pumping and dissipation processes for a single atom. (b) Multi-atom arrangement and laser polarization direction for a single atom. (c) Pulse driving sequence, with the two 480 nm laser pulses repeated \(\mathcal{N}\) times shown as a representative sketch. The colors in the subfigures consistently represent the distinct characteristics of the pulses.} \label{fig_doppler}
\end{figure}

We provide a detailed description of the experimental implementation. Our approach has two primary objectives: first, to employ maximally circularly polarized light to ensure uniform atomic phases, thereby simplifying the system dynamics; second, to maximize dissipation toward the \( |0\rangle \) state. The Hamiltonians in Eqs.~(\ref{eq:H_S1})--(\ref{eq:H_Sk}) indicate that the \( |1_i\rangle \) component is volatile, whereas the \( |0_i\rangle \) component remains relatively quiescent. By engineering dissipation directly to the \( |0\rangle \) state, we achieve the fastest convergence to the target entangled state.

To this end, we select the stretched ground state \( |0\rangle \equiv |5S_{1/2}, F=2, m_F=2\rangle \) and the clock ground state \( |1\rangle \equiv |5S_{1/2}, F=1, m_F=0\rangle \). The Rydberg state is chosen as \( |r\rangle \equiv |79D_{5/2}, m_j=5/2\rangle \). For two-photon excitation, we utilize an intermediate state \( |p'\rangle \equiv |5P_{3/2}, F=2, m_F=1\rangle \), while for engineered dissipation, we use another intermediate state \( |p\rangle \equiv |5P_{3/2}, F=3, m_F=3\rangle \), which decays exclusively to the \( |0\rangle \) state due to transition selection rules. Specific details, including polarization and wavelength, are depicted in Fig.~\ref{fig_doppler}(a) and \ref{fig_doppler}(b). The pulse sequence is illustrated in Fig.~\ref{fig_doppler}(c), where the driving fields with Rabi frequencies \( \Omega_{0p'} \) and \( \Omega_{1p'} \) are selectively activated based on the excited stabilizers.

\bibliography{SM.bbl}

\end{document}
